# Supplementary material for: Improving the Robustness of 3D Human Pose Estimation: A Benchmark and Learning from Noisy Input
Source: arXiv:2312.06797 source file (2024-04-16)
Supplement: Supplementary file 1 [file supplementary.tex]

\section{Temporal Additive Gaussian Noise}

Algorithm \ref{alg:additive_gauss_noise} elaborates upon our proposed Temporal Additive Gaussian Noise (TAGN) strategy.

\begin{algorithm}[H]
    \KwIn{Keypoints sequence $\mathbf{x} (t) \in \mathbb{R}^{|\mathcal{J}| \times 2}$, temporal distortion ratio $k\%$, joint distortion ratio $p\%$, noise variance $\sigma^2$, set of frame indices $\mathcal{T}$, set of joints indices $\mathcal{J}$} 
    
    \tcp{Uniformly select k\% of frames}
    $\Tilde{\mathcal{T}} \leftarrow \text{Choice}(\mathcal{T}, k)$ \tcp{Set of distorted frames} 
    
    $\mathbf{\Tilde{x}} \leftarrow \mathbf{x}$ \tcp{Initialize }   
    
    \For{$t \in \Tilde{\mathcal{T}}$}{
        \tcp{Uniformly select p\% of joints}
        $\Tilde{\mathcal{J}}_t \leftarrow \text{Choice}(\mathcal{J}, p)$ \tcp{Set of distorted joints at frame t}
    
        \For{$j \in \Tilde{\mathcal{J}}_t$}{
        \tcp{Add noise}
            $\mathbf{\Tilde{x}}_j(t) \leftarrow \mathbf{x}_j(t) + \varepsilon, \,\, \varepsilon \sim \mathcal{N}(0, \sigma^2)$
        }
    }
    \tcp{Return distorted keypoints}
    \KwOut{$\mathbf{\Tilde{x}}$} 
    \caption{Temporal Additive Gaussian Noise (TAGN)}
    \label{alg:additive_gauss_noise}
\end{algorithm}

\section{Implementation Details}
\subsection{Video Corruption Operators}

\noindent \textbf{Guided-patch Erasing (GPE):} Given a video, the masking patch positions are selected such that they have the most overlap with a selected keypoints' trajectory. We perform $K$-means clustering ($K$ is randomly selected from $\{2,3,4\}$) over the set of all aggregated keypoint locations throughout the input video to find the centroids of the $K$-clusters. These centroids would then mark the center of the masking patches. Finally, GPE deletes $K$ square patches with the fixed size of $\lfloor \frac{\min{(W,H)}}{10} \rfloor$ ($W$ and $H$ denoting the width and height of a frame, respectively).

\noindent \textbf{Cropping: } We perform horizontal cropping over the original video. The cut-off location is determined according to the average of all keypoints' horizontal positions ($y_{\text{avg}}$). However, to ensure the cut-off not making the aspect ratio too small, we limit its value by $\min (y_{\text{avg}}, 2H/3)$. Finally, the cropped images are resized to the original resolution of the dataset.

\noindent \textbf{Gaussian \& Impulse Noise: } Following \cite{hendrycks2018benchmarking} and adhering to their settings, we perturb the video frames using Gaussian and impulse noise. We randomly inject zero-mean Gaussian noise with $\sigma=0.38$ over all pixels at each frame in the original video. For the impulse noise, we randomly add impulse noise to $27\%$ of the pixels at each frame.

\noindent \textbf{Motion Blur: }We utilize the motion blur kernel implemented by \cite{hendrycks2018benchmarking}. This distortion emulates the blurring effect caused by a fast moving subject or camera, by applying a shifted Gaussian kernel specified by the angle of the shifting operation ($\theta$) and its standard deviation along horizontal and vertical axes ($\delta$). In this paper, we chose $\theta \sim \text{Uniform}(-\pi /4, \pi /4)$ and $\delta=\left[20, 15\right]^{T}$.

In Figure \ref{fig:dataset}, we provide frame samples of the H36M-C and HumanEva-I-C datasets, to better visualize the effect of each video corruption operator. 

\begin{figure*}[t!]
    \pgfplotsset{every x tick label/.append style={font=\tiny, yshift=0.5ex}}
    \pgfplotsset{every y tick label/.append style={font=\tiny, xshift=0.5ex}}
    \centering
    
        \hspace{-10pt}
        \begin{tikzpicture}
        \def \h{2.15}
        \def \w{2.10}
        \def \imgw{2.0cm}

        \def \r{0} 
        \node at (-1.5, 0,\h * \r) [below, rotate=90] {\footnotesize{Motion Blur}};
        \node at (-1.5, \h * 1, \h * \r) [below, rotate=90] {\footnotesize{Impulse Noise}};
        \node at (-1.5, \h * 2, \h * \r) [below, rotate=90] {\footnotesize{Gaussian Noise}};
        \node at (-1.5, \h * 3,  \h * \r) [below, rotate=90] {\footnotesize{Cropping}};
        \node at (-1.5, \h * 4,  \h * \r) [below, rotate=90] {\footnotesize{GPE}};
        \draw (\w * 0, \h * \r) node[inner sep=0] {\includegraphics[width=\imgw]{resources/dataset_samples/motion_blur_1.png}};
        \draw (\w * 1, \h * \r)node[inner sep=0]  {\includegraphics[width=\imgw]{resources/dataset_samples/motion_blur_2.png}};
        \draw (\w * 2, \h * \r) node[inner sep=0] {\includegraphics[width=\imgw]{resources/dataset_samples/motion_blur_3.png}};
        \draw (\w * 3 ,\h * \r) node[inner sep=0] {\includegraphics[width=\imgw]{resources/dataset_samples/motion_blur_4.png}};
        \draw (\w * 4, \h * \r) node[inner sep=0] {\includegraphics[width=\imgw]{resources/dataset_samples/motion_blur_5.png}};
        \draw (\w * 5, \h * \r) node[inner sep=0] {\includegraphics[width=\imgw]{resources/dataset_samples/motion_blur_6.png}};
        \draw (\w * 6, \h * \r) node[inner sep=0] {\includegraphics[width=\imgw]{resources/dataset_samples/motion_blur_7.png}};
        \draw (\w * 7, \h * \r) node[inner sep=0] {\includegraphics[width=\imgw]{resources/dataset_samples/motion_blur_8.png}};
        
        \def \r{1} 
        \draw (\w * 0, \h * \r) node[inner sep=0] {\includegraphics[width=\imgw]{resources/dataset_samples/impulse_noise_1.jpg}};
        \draw (\w * 1, \h * \r)node[inner sep=0]  {\includegraphics[width=\imgw]{resources/dataset_samples/impulse_noise_2.jpg}};
        \draw (\w * 2, \h * \r) node[inner sep=0] {\includegraphics[width=\imgw]{resources/dataset_samples/impulse_noise_3.png}};
        \draw (\w * 3 ,\h * \r) node[inner sep=0] {\includegraphics[width=\imgw]{resources/dataset_samples/impulse_noise_4.png}};
        \draw (\w * 4, \h * \r) node[inner sep=0] {\includegraphics[width=\imgw]{resources/dataset_samples/impulse_noise_5.png}};
        \draw (\w * 5, \h * \r) node[inner sep=0] {\includegraphics[width=\imgw]{resources/dataset_samples/impulse_noise_6.png}};
        \draw (\w * 6, \h * \r) node[inner sep=0] {\includegraphics[width=\imgw]{resources/dataset_samples/impulse_noise_7.png}};
        \draw (\w * 7, \h * \r) node[inner sep=0] {\includegraphics[width=\imgw]{resources/dataset_samples/impulse_noise_8.png}};
        
        \def \r{2} 
        \draw (\w * 0, \h * \r) node[inner sep=0] {\includegraphics[width=\imgw]{resources/dataset_samples/gaussian_noise_1.png}};
        \draw (\w * 1, \h * \r)node[inner sep=0]  {\includegraphics[width=\imgw]{resources/dataset_samples/gaussian_noise_2.png}};
        \draw (\w * 2, \h * \r) node[inner sep=0] {\includegraphics[width=\imgw]{resources/dataset_samples/gaussian_noise_3.png}};
        \draw (\w * 3 ,\h * \r) node[inner sep=0] {\includegraphics[width=\imgw]{resources/dataset_samples/gaussian_noise_4.png}};
        \draw (\w * 4, \h * \r) node[inner sep=0] {\includegraphics[width=\imgw]{resources/dataset_samples/gaussian_noise_5.png}};
        \draw (\w * 5, \h * \r) node[inner sep=0] {\includegraphics[width=\imgw]{resources/dataset_samples/gaussian_noise_6.png}};
        \draw (\w * 6, \h * \r) node[inner sep=0] {\includegraphics[width=\imgw]{resources/dataset_samples/gaussian_noise_7.png}};
        \draw (\w * 7, \h * \r) node[inner sep=0] {\includegraphics[width=\imgw]{resources/dataset_samples/gaussian_noise_8.png}};
        
        \def \r{3} 
        \draw (\w * 0, \h * \r) node[inner sep=0] {\includegraphics[width=\imgw]{resources/dataset_samples/crop_1.png}};
        \draw (\w * 1, \h * \r)node[inner sep=0]  {\includegraphics[width=\imgw]{resources/dataset_samples/crop_2.png}};
        \draw (\w * 2, \h * \r) node[inner sep=0] {\includegraphics[width=\imgw]{resources/dataset_samples/crop_3.png}};
        \draw (\w * 3 ,\h * \r) node[inner sep=0] {\includegraphics[width=\imgw]{resources/dataset_samples/crop_4.png}};
        \draw (\w * 4, \h * \r) node[inner sep=0] {\includegraphics[width=\imgw]{resources/dataset_samples/crop_5.png}};
        \draw (\w * 5, \h * \r) node[inner sep=0] {\includegraphics[width=\imgw]{resources/dataset_samples/crop_6.png}};
        \draw (\w * 6, \h * \r) node[inner sep=0] {\includegraphics[width=\imgw]{resources/dataset_samples/crop_7.png}};
        \draw (\w * 7, \h * \r) node[inner sep=0] {\includegraphics[width=\imgw]{resources/dataset_samples/crop_8.png}};
        
        \def \r{4} 
        \draw (\w * 0, \h * \r) node[inner sep=0] {\includegraphics[width=\imgw]{resources/dataset_samples/erase_1.png}};
        \draw (\w * 1, \h * \r)node[inner sep=0]  {\includegraphics[width=\imgw]{resources/dataset_samples/erase_2.png}};
        \draw (\w * 2, \h * \r) node[inner sep=0] {\includegraphics[width=\imgw]{resources/dataset_samples/erase_3.png}};
        \draw (\w * 3 ,\h * \r) node[inner sep=0] {\includegraphics[width=\imgw]{resources/dataset_samples/erase_4.png}};
        \draw (\w * 4, \h * \r) node[inner sep=0] {\includegraphics[width=\imgw]{resources/dataset_samples/erase_8.jpg}};
        \draw (\w * 5, \h * \r) node[inner sep=0] {\includegraphics[width=\imgw]{resources/dataset_samples/erase_6.png}};
        \draw (\w * 6, \h * \r) node[inner sep=0] {\includegraphics[width=\imgw]{resources/dataset_samples/erase_7.png}};
        \draw (\w * 7, \h * \r) node[inner sep=0] {\includegraphics[width=\imgw]{resources/dataset_samples/erase_5.png}};

        \end{tikzpicture}
    \caption{Examples of H36M-C (first five columns from the left) and HumanEva-I-C (last three columns from the left) dataset. Each row corresponds to samples obtained under different video corruption operators.}
    \vspace*{-\baselineskip}
    \label{fig:dataset}
\end{figure*}

\subsection{Baseline Models}
All baselines are optimized using Adam optimizer \cite{kingma2015_adam} with a learning rate $0.001$, step decay $0.95$, and batch-size equal to $1024$, unless otherwise stated. We train Pose3D-RIE for $240$ and the rest of the baselines for $80$ epochs. All baselines are implemented in PyTorch and trained on a single GPU (except for PoseFormer \cite{zheng2021_poseformer} and Pose3D-RIE \cite{shan2021improving}).

\noindent \textbf{VideoPose3D (VP3D) \cite{pavllo2019_videopose3d}}: We trained VP3D models with various receptive fields of $1$, $3$, $9$ and $27$. For the single frame model (i.e. receptive field size of $1$), we use $B=3$ convolution blocks, each with kernel size $K=1$. We keep the number of intermediate channels as $C=1024$. For VP3D models with receptive field $\geq 1$, the kernel size of all convolution blocks is $K=3$. For models with a receptive field of size $3^m$, $m \geq 1$, the number of convolution blocks is $m$. We also set the dropout rate as $25\%$.

\noindent \textbf{SRNet \cite{zeng2020_srnet}}: We used the proposed split-and-recombine model. For better comparability, we select the same architecture as VP3D, with $B=3$ convolution blocks and a receptive field of $27$ frames.

\noindent \textbf{PoseFormer \cite{zheng2021_poseformer}}: We adopted a PoseFormer model with 27 frames receptive field. The spatial and temporal transformers both consist of $4$ blocks and the stochastic depth rate \cite{huang2016_stochastic} is set to $10\%$ during training. Additionally, the token embedding size is set to $32$ while the number of heads is $8$.  We used $4 \times$A100 GPUs for training in parallel with a batch size of 256 on each single GPU. 

\noindent \textbf{Attention3DHP \cite{liu2020_attention}}: We employed an Attention3DHP model with 243-frame receptive field and $C=1024$ intermediate channels. For this baseline, we chose a batch size of 2048.

\noindent \textbf{Pose3D-RIE \cite{shan2021improving}}: Following \cite{shan2021improving}, we use a 3-stage optimization pipeline, run for a total of $240$ epochs to fully exploit the positional and temporal information in human keypoint groups. The encoder and the feature fusion module (FFM) is trained in the first stage. In the second stage, only the FFM and decoder are optimized. Finally, the parameters of the entire framework is fine-tuned with a small learning rate in the third stage. For a fair comparison with other single stage baselines, we used a receptive field size of $27$ instead of $243$ frames, as originally used by \cite{shan2021improving}. Meanwhile, we keep the latent feature dimension of $256$ and use a smaller learning rate of $0.0005$ similar to~\cite{shan2021improving}. We used $4 \times$A100 GPUs for training in parallel, with an effective batch size of $2048$.

\subsection{2D Keypoint Detectors}
We use HRNet \cite{sun2019_hrnet} and LiteHRnet \cite{yu2021_lite-hrnet} for the 2D keypoint detection. Both 2D pose estimators are top-down solutions requiring a human detector. In our experiments with H36M-C, we found that a simple Faster-RCNN \cite{Ren2015FasterRT} with a ResNet-50 \cite{He2016DeepRL} and feature pyramid network backbone trained \cite{Lin2017FeaturePN} on COCO \cite{lin2014_coco} performs well on the human detection task. We used HRNet-W48 and LiteHRNet-18 both trained on COCO with input image size of $256\times 192$. The specific configurations of the 2D keypoint detectors can be found in the MMPose framework\cite{mmpose2020}.
\begin{figure}[t]
    \centering
    \input{resources/mpjpe01_cdf}
    \caption{Percentage of joints (per frame) involved in deriving MPJPE$_{\leq \tau}$ as a function of the threshold $\tau$. The results are reported on H36M-C test set.}
    \label{fig:mpjpe_cdf}
    \vspace*{-\baselineskip}
\end{figure}

\section{Experimental Results}
\begin{table*}[t!]
  \caption{Comparison between various baselines trained with TAGN. The mean and standard deviation across $5$ random runs are reported.}
  \label{tab:supp_mpjpe-tagn}
  \centering
    \resizebox{\linewidth}{!}{
    \begin{tabular}{@{}l|cccccc|c@{}}
    \toprule
    \multicolumn{1}{c|}{\textbf{Model}} & \textbf{\begin{tabular}[c]{@{}c@{}}Gaussian \\ Noise\end{tabular}} & \textbf{\begin{tabular}[c]{@{}c@{}}Impulse \\ Noise\end{tabular}} & \textbf{\begin{tabular}[c]{@{}c@{}}Temporal-patch \\ Erasing\end{tabular}} &  \textbf{\begin{tabular}[c]{@{}c@{}}Guided-patch \\ Erasing\end{tabular}} & \textbf{Cropping} & \textbf{\begin{tabular}[c]{@{}c@{}}Motion \\ Blur\end{tabular}} & \textbf{Average} \\ \midrule
    \hline
    VP3D\cite{pavllo2019_videopose3d}/H36M+\textit{TAGN} ($\sigma=0.05; p=k=20\%$)  
         & $91.73 \pm 0.30$ & $94.12 \pm 0.32$ & $96.08 \pm 0.38$ & $112.72 \pm 0.56$ & $117.23 \pm 1.09$ & $76.54 \pm 0.24$ & $98.07 \pm 0.48$ 
    \\
    VP3D\cite{pavllo2019_videopose3d}/H36M+\textit{TAGN} ($\sigma=0.1; p=k=30\%$) 
         & $88.44 \pm 0.35$ & $90.69 \pm 0.35$ & $93.56 \pm 0.13$ & $108.95 \pm 0.22$ & $114.30 \pm 0.68$ & $75.38 \pm 0.09$ & $95.22 \pm 0.30$ 
    \\
    VP3D\cite{pavllo2019_videopose3d}/H36M+\textit{TAGN} ($\sigma=0.3; p=k=50\%$) 
         & $86.30 \pm 0.27$ & $88.46 \pm 0.27$ & $92.57 \pm 0.33$ & $106.74 \pm 0.65$ & $107.71 \pm 0.54$ & $75.89 \pm 0.16$ & $92.94 \pm 0.37$ 
    \\

    \hline
    PoseFormer\cite{zheng2021_poseformer}/H36M+\textit{TAGN} ($\sigma=0.3; p=k=50\%$) 
        & $102.24 \pm 4.03$ & $104.78 \pm 4.13$ & $113.80 \pm 3.67$ & $129.33 \pm 3.67$ & $148.39 \pm 7.11$ & $88.70 \pm 4.31$ & $114.54 \pm 4.49$ \\
    
    SRNet\cite{zeng2020_srnet}/H36M+\textit{TAGN} ($\sigma=0.3; p=k=50\%$)
         & $91.68 \pm 1.32$ & $94.04 \pm 1.49$ & $96.16 \pm 0.82$ & $111.94 \pm 0.90$ & $117.28 \pm 3.18$ & $78.70 \pm 0.59$ & $98.30 \pm 1.38$ 
        \\
    
    Attention3DHP\cite{liu2020_attention}/H36M+\textit{TAGN} ($\sigma=0.3; p=k=50\%$) 
        & $92.05 \pm 0.77$ & $93.94 \pm 0.90 $ & $100.48 \pm 1.12 $ & $115.08 \pm 1.13$ & $112.80 \pm 1.52$ & $84.35 \pm 0.81$ & $99.78 \pm 1.04$ \\
    
    Pose3D-RIE\cite{shan2021improving}/H36M+\textit{TAGN} ($\sigma=0.3; p=k=50\%$) 
         & $92.14 \pm 1.15$   & $101.34 \pm 0.23$ & $105.45 \pm 1.13$  & $115.31 \pm 0.34$  & $104.42 \pm 0.12$  & $92.40 \pm 1.62$  & $101.84 \pm 0.68$ \\
    \bottomrule
    \end{tabular}
    }
\end{table*}

\begin{table*}[t!]
  \caption{Effect of TAGN on $\text{MPJPE}_{\leq 0.1}$ of VP3D \cite{pavllo2019_videopose3d} models trained/tested on 2D keypoints detected by HRNet\cite{sun2019_hrnet} and Lite-HRNet \cite{yu2021_lite-hrnet}. The mean and standard deviations across $5$ random runs are reported.}
  \label{tab:supp_mpjpe_tagn-hrnet-lite-hrnet}
  \centering
    \resizebox{\linewidth}{!}{
    \begin{tabular}{@{}c|c|l|cccccc|c@{}}
    \toprule
    \textbf{\begin{tabular}[c]{@{}c@{}}Training \\ Keypoints \end{tabular}} & \textbf{\begin{tabular}[c]{@{}c@{}}Testing \\ Keypoints \end{tabular}} & \multicolumn{1}{c|}{ \textbf{Model}} & \textbf{\begin{tabular}[c]{@{}c@{}}Gaussian \\ Noise\end{tabular}} & \textbf{\begin{tabular}[c]{@{}c@{}}Impulse \\ Noise\end{tabular}} & \textbf{\begin{tabular}[c]{@{}c@{}}Temporal-patch \\ Erasing\end{tabular}} &  \textbf{\begin{tabular}[c]{@{}c@{}}Guided-patch \\ Erasing\end{tabular}} & \textbf{Cropping} & \textbf{\begin{tabular}[c]{@{}c@{}}Motion \\ Blur\end{tabular}} & \textbf{Average} \\ \midrule
    HRNet & HRNet & VP3D\cite{pavllo2019_videopose3d}     
        &  94.27& 96.64 & 99.32 & 116.54 & 118.08 &  78.14 & 100.50
    \\
    HRNet & HRNet & VP3D\cite{pavllo2019_videopose3d}+{TAGN}
        & $86.30 \pm 0.27$ & $88.46 \pm 0.27$ & $92.57 \pm 0.33$ & $106.74 \pm 0.65$ & $107.71 \pm 0.54$ & $75.89 \pm 0.16$ & $92.94 \pm 0.37$
    \\
    
    \midrule
    
    HRNet & Lite-HRNet & VP3D\cite{pavllo2019_videopose3d}
        & $123.69$ & $127.27$ & $118.76$ & $132.68$ & $116.56$ & $91.76$ & $118.45$ 
    \\
    HRNet & Lite-HRNet & VP3D\cite{pavllo2019_videopose3d}+{TAGN}
        & $121.78 \pm 0.25$ & $125.04 \pm 0.28$ & $110.21 \pm 0.36$ & $121.85 \pm 0.73$ & $107.11 \pm 0.76$ & $87.59 \pm 0.16$ & $112.26 \pm 0.42$
    \\
    
    \hline
    \midrule
    
    Lite-HRNet & HRNet & VP3D\cite{pavllo2019_videopose3d}
        & $94.32 $ & $96.76 $ & $101.47 $ & $118.77 $ & $121.07 $ & $77.56 $ & $101.66 $ 
    \\
    Lite-HRNet & HRNet & VP3D\cite{pavllo2019_videopose3d}+{TAGN}
        & $91.73 \pm 0.30$ & $94.12 \pm 0.32$ & $96.08 \pm 0.38$ & $112.72 \pm 0.56$ & $117.23 \pm 1.09$ & $76.54 \pm 0.24$ & $98.07 \pm 0.48$ 
    \\
    
    \midrule
    
    Lite-HRNet & Lite-HRNet & VP3D\cite{pavllo2019_videopose3d}
        & $120.30 $ & $123.76 $ & $116.66 $ & $130.20 $ & $116.80 $ & $87.94 $ & $115.94 $ 
    \\
    Lite-HRNet & Lite-HRNet & VP3D\cite{pavllo2019_videopose3d}+{TAGN}
        & $85.82 \pm 0.33$ & $88.05 \pm 0.33$ & $95.73 \pm 0.24$ & $110.03 \pm 0.30$ & $109.13 \pm 1.05$ & $76.19 \pm 0.17$ & $94.16 \pm 0.40$ 
    \\
    
    \bottomrule
    \end{tabular}
    }
\end{table*}

\begin{table*}[t!]
  \caption{Effect of CA-Conv block on $\text{MPJPE}_{\leq 0.1}$ of VP3D\cite{pavllo2019_videopose3d} models trained/tested on 2D keypoints detected by HRNet \cite{sun2019_hrnet} and Lite-HRNet \cite{yu2021_lite-hrnet}.}
  \label{tab:supp_mpjpe_ca-conv-hrnet-lite-hrnet}
  \centering
    \resizebox{\linewidth}{!}{
    \begin{tabular}{@{}c|c|l|cccccc|c@{}}
    \toprule
    \textbf{\begin{tabular}[c]{@{}c@{}}Training \\ Keypoints \end{tabular}} & \textbf{\begin{tabular}[c]{@{}c@{}}Testing \\ Keypoints \end{tabular}} & \multicolumn{1}{c|}{ \textbf{Model}} & \textbf{\begin{tabular}[c]{@{}c@{}}Gaussian \\ Noise\end{tabular}} & \textbf{\begin{tabular}[c]{@{}c@{}}Impulse \\ Noise\end{tabular}} & \textbf{\begin{tabular}[c]{@{}c@{}}Temporal-patch \\ Erasing\end{tabular}} &  \textbf{\begin{tabular}[c]{@{}c@{}}Guided-patch \\ Erasing\end{tabular}} & \textbf{Cropping} & \textbf{\begin{tabular}[c]{@{}c@{}}Motion \\ Blur\end{tabular}} & \textbf{Average} \\ \midrule
    HRNet & HRNet & VP3D\cite{pavllo2019_videopose3d}     
       & $73.11 $ & $74.03 $ & $81.65 $ & $90.56 $ & $79.76 $ & $68.40 $ & $77.92 $ 
    \\
    HRNet & HRNet & VP3D\cite{pavllo2019_videopose3d}+{CA-Conv}
       & $72.31 $ & $73.28 $ & $79.45 $ & $87.72 $ & $76.84 $ & $67.16 $ & $76.13 $
    \\
    
    \midrule
    
    HRNet & Lite-HRNet & VP3D\cite{pavllo2019_videopose3d}
       & $105.71 $ & $109.93 $ & $101.01 $ & $107.46 $ & $83.36 $ & $80.71 $ & $98.03 $ 
    \\
    HRNet & Lite-HRNet & VP3D\cite{pavllo2019_videopose3d}+{CA-Conv}
        & $107.72 $ & $111.27 $ & $101.56 $ & $107.20 $ & $83.92 $ & $84.17 $ & $99.31 $ 
    \\
    
    \hline
    \midrule
    
    Lite-HRNet & HRNet & VP3D\cite{pavllo2019_videopose3d}
        & $78.21 $ & $80.34 $ & $87.56 $ & $97.35 $ & $89.27 $ & $71.77 $ & $84.08 $ 
    \\
    Lite-HRNet & HRNet & VP3D\cite{pavllo2019_videopose3d}+{CA-Conv}
        & $75.24 $ & $77.49 $ & $84.49 $ & $93.92 $ & $88.86 $ & $69.52 $ & $81.59 $ 
    \\
    
    \midrule
    
    Lite-HRNet & Lite-HRNet & VP3D\cite{pavllo2019_videopose3d}
        & $91.60 $ & $91.89 $ & $97.96 $ & $103.43 $ & $86.79 $ & $79.12 $ & $91.80 $ 
    \\
    Lite-HRNet & Lite-HRNet & VP3D\cite{pavllo2019_videopose3d}+{CA-Conv}
        & $88.24 $ & $88.31 $ & $95.35 $ & $100.66 $ & $84.97 $ & $76.51 $ & $89.01 $
    \\
    \bottomrule
    \end{tabular}
    }
\end{table*}

\begin{table*}[t!]
  \caption{Effect of receptive field on $\text{MPJPE}_{\leq 0.1}$ of VP3D models trained with and without TAGN. The mean and standard deviations across $5$ random runs are reported.}
  \label{tab:supp_mpjpe-tagn-receptive-field}
  \centering
    \resizebox{\linewidth}{!}{
    \begin{tabular}{@{}c|l|cccccc|c@{}}
    \toprule
    \textbf{\begin{tabular}[c]{@{}c@{}}Receptive \\ Field \end{tabular}} & \multicolumn{1}{c|}{ \textbf{Model}} & \textbf{\begin{tabular}[c]{@{}c@{}}Gaussian \\ Noise\end{tabular}} & \textbf{\begin{tabular}[c]{@{}c@{}}Impulse \\ Noise\end{tabular}} & \textbf{\begin{tabular}[c]{@{}c@{}}Temporal-patch \\ Erasing\end{tabular}} &  \textbf{\begin{tabular}[c]{@{}c@{}}Guided-patch \\ Erasing\end{tabular}} & \textbf{Cropping} & \textbf{\begin{tabular}[c]{@{}c@{}}Motion \\ Blur\end{tabular}} & \textbf{Average} \\ \midrule
    1 & VP3D\cite{pavllo2019_videopose3d}     
        & $97.80 $ & $100.06 $ & $102.80 $ & $119.24 $ & $119.00 $ & $80.39 $ & $103.22 $ 
    \\
    1 & VP3D \cite{pavllo2019_videopose3d} + {TAGN}
        & $94.98 \pm 0.09$ & $96.87 \pm 0.10$ & $94.95 \pm 0.08$ & $107.69 \pm 0.14$ & $102.16 \pm 0.62$ & $80.26 \pm 0.14$ & $96.15 \pm 0.19$ 
    \\
    \hline
    9 & VP3D\cite{pavllo2019_videopose3d}     
        & $96.61 $ & $99.11 $ & $101.95 $ & $119.03 $ & $118.85 $ & $80.92 $ & $102.74 $
    \\
    9 & VP3D \cite{pavllo2019_videopose3d} + {TAGN}
       & $93.08 \pm 0.40$ & $94.95 \pm 0.45$ & $96.69 \pm 0.21$ & $110.26 \pm 0.37$ & $107.86 \pm 0.77$ & $81.25 \pm 0.23$ & $97.35 \pm 0.40$
    \\
    \hline
    27 & VP3D\cite{pavllo2019_videopose3d}     
       & $94.27 $ & $96.64 $ & $99.32 $ & $116.54 $ & $118.08 $ & $78.14 $ & $100.50 $
    \\
    27 & VP3D \cite{pavllo2019_videopose3d} + {TAGN}
        & $86.30 \pm 0.27$ & $88.46 \pm 0.27$ & $92.57 \pm 0.33$ & $106.74 \pm 0.65$ & $107.71 \pm 0.54$ & $75.89 \pm 0.16$ & $92.94 \pm 0.37$ 
    \\
    \hline
    81 & VP3D\cite{pavllo2019_videopose3d}     
        & $93.14 $ & $95.73 $ & $97.34 $ & $114.60 $ & $120.78 $ & $76.54 $ & $99.69 $ 
    \\
    81 & VP3D \cite{pavllo2019_videopose3d} + {TAGN}
        & $84.61 \pm 0.37$ & $86.67 \pm 0.41$ & $91.36 \pm 0.20$ & $105.75 \pm 0.38$ & $106.92 \pm 0.51$ & $75.16 \pm 0.16$ & $91.74 \pm 0.34$ 
    \\
    \bottomrule
    \end{tabular}
    }
\end{table*}

\begin{table*}[t!]
  \caption{Effect of VP3D \cite{pavllo2019_videopose3d}'s receptive field on $\text{MPJPE}_{\leq 0.1}$ of VP3D models trained with CA-Conv}
  \label{tab:supp_mpjpe-ca-conv-receptive-field}
  \centering
    \resizebox{0.9\linewidth}{!}{
    \begin{tabular}{@{}c|l|cccccc|c@{}}
    \toprule
    \textbf{\begin{tabular}[c]{@{}c@{}}Receptive \\ Field \end{tabular}} & \multicolumn{1}{c|}{ \textbf{Model}} & \textbf{\begin{tabular}[c]{@{}c@{}}Gaussian \\ Noise\end{tabular}} & \textbf{\begin{tabular}[c]{@{}c@{}}Impulse \\ Noise\end{tabular}} & \textbf{\begin{tabular}[c]{@{}c@{}}Temporal-patch \\ Erasing\end{tabular}} &  \textbf{\begin{tabular}[c]{@{}c@{}}Guided-patch \\ Erasing\end{tabular}} & \textbf{Cropping} & \textbf{\begin{tabular}[c]{@{}c@{}}Motion \\ Blur\end{tabular}} & \textbf{Average} \\ \midrule
    1 & VP3D\cite{pavllo2019_videopose3d}     
         & $86.96 $ & $87.96 $ & $87.75 $ & $96.52 $ & $81.05 $ & $76.61 $ & $86.14 $
    \\
    1 & VP3D \cite{pavllo2019_videopose3d} + {CA-Conv}
       & $85.21 $ & $86.16 $ & $84.16 $ & $92.16 $ & $77.14 $ & $74.85 $ & $83.28 $ 
    \\
    \hline
    9 & VP3D\cite{pavllo2019_videopose3d}     
        & $78.11 $ & $79.27 $ & $85.68 $ & $94.57 $ & $83.53 $ & $71.92 $ & $82.18 $ 
    \\
    9 & VP3D \cite{pavllo2019_videopose3d} + {CA-Conv}
        & $76.68 $ & $77.58 $ & $82.96 $ & $91.61 $ & $79.53 $ & $69.92 $ & $79.71 $ 
    \\
    \hline
    27 & VP3D\cite{pavllo2019_videopose3d}     
        & $73.11 $ & $74.03 $ & $81.65 $ & $90.56 $ & $79.76 $ & $68.40 $ & $77.92 $ 
    \\
    27 & VP3D \cite{pavllo2019_videopose3d} + {CA-Conv}
        & $72.31 $ & $73.28 $ & $79.45 $ & $87.72 $ & $76.84 $ & $67.16 $ & $76.13 $ 
    \\
    \hline
    81 & VP3D\cite{pavllo2019_videopose3d}     
        & $70.85 $ & $71.82 $ & $79.55 $ & $87.83 $ & $77.94 $ & $66.78 $ & $75.80 $ 
    \\
    81 & VP3D \cite{pavllo2019_videopose3d} + {CA-Conv}
        & $69.92 $ & $70.91 $ & $77.02 $ & $85.23 $ & $76.24 $ & $65.42 $ & $74.12 $ 
    \\
    \bottomrule
    \end{tabular}
    }
\end{table*}

In Figure \ref{fig:mpjpe_cdf}, we evaluate the effect of the threshold $\tau$ on the number of joints considered when computing the MPJPE$_{\leq \tau}$ metric. As expected, with a larger threshold, more joints are included in the computation of MPJPE$_{\leq \tau}$. In our experiments, we selected a default value of $\tau\!=\!0.1$ which captures $87\%$ of the total joints. 

To showcase the consistency of the performance of TAGN, in Table \ref{tab:supp_mpjpe-tagn}, \ref{tab:supp_mpjpe_tagn-hrnet-lite-hrnet}, and \ref{tab:supp_mpjpe-tagn-receptive-field}, we report the mean and standard deviation across $5$ random runs. Note that, in each run, we have different noise realizations added by TAGN to the 2D input pose. The small standard deviations affirm the stable boost in performance, offered by TAGN. 

\begin{figure}[t]
    \centering
    \includegraphics[width=\linewidth]{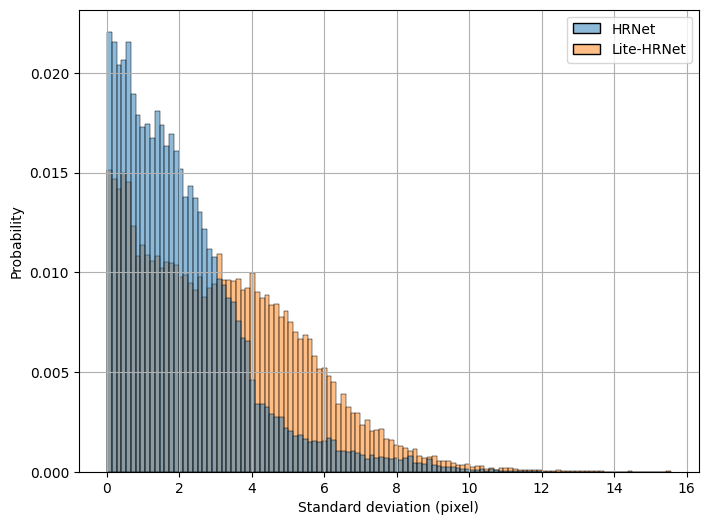}
    \vspace*{-0.5\baselineskip} 
    \caption{Histogram of the standard deviation of the heatmaps around 2D keypoint predictions of one subject (H36M dataset) from HRNet~\cite{sun2019_hrnet} and Lite-HRNet~\cite{yu2021_lite-hrnet}. The confidence score of each detected 2D keypoint corresponds to the maximum of the associated heatmap.}
    \label{fig:hrnet-lite-hrnet}
    \vspace*{-1.5\baselineskip}
\end{figure}

In Figure \ref{fig:hrnet-lite-hrnet}, we provide the histogram of the standard deviation of output heatmaps around all 2D keypoint predictions of one subject from HRNet~\cite{sun2019_hrnet} and Lite-HRNet~\cite{yu2021_lite-hrnet}. We notice the difference between the two distributions produced by HRNet and Lite-HRNet. In general, HRNet predicts not only more accurate but also more confident keypoints than Lite-HRNet. 

Furthermore, in Table \ref{tab:supp_mpjpe_tagn-hrnet-lite-hrnet} and \ref{tab:supp_mpjpe_ca-conv-hrnet-lite-hrnet}, we study VP3D~\cite{pavllo2019_videopose3d} trained with TAGN or CA-Conv, with 2D pose output by HRNet and LiteHRNet. Similarly, Table \ref{tab:supp_mpjpe-tagn-receptive-field} and \ref{tab:supp_mpjpe-ca-conv-receptive-field} summarize the effect of receptive field size on VP3D's ~\cite{pavllo2019_videopose3d} performance. In all scenarios, our proposed TAGN and CA-Conv solutions lead to improvements in MPJPE$_{\leq \tau}$ compared to the upper and lower-bound benchmarks. 

\begin{figure*}[t!]
    \pgfplotsset{every x tick label/.append style={font=\tiny, yshift=0.5ex}}
    \pgfplotsset{every y tick label/.append style={font=\tiny, xshift=0.5ex}}
    \centering
    
        \hspace{-10pt}
        \begin{tikzpicture}
        \def \h{6.5}
        \def \u{0.6}
        \def \w{1.65}

        \def \r{0} 
        \node at (-1.5,\u * -4 , \h * \r) [below, rotate=90] {\footnotesize{VP3D + }};
        \node at (-1.25, \u * -4,\h * \r) [below, rotate=90] {\footnotesize{TAGN}};
        \node at (-1.375, \u * -1.5, \h * \r) [below, rotate=90] {\footnotesize{VP3D}};
        \node at (-1.375, \u * 1.2,  \h * \r) [below, rotate=90] {\footnotesize{GT}};
        \node at (-1.375, \u * 4,  \h * \r) [below, rotate=90] {\footnotesize{Frame}};
        \draw (\w * 0, \h * \r) node[inner sep=0] {\includegraphics[width=1.57cm]{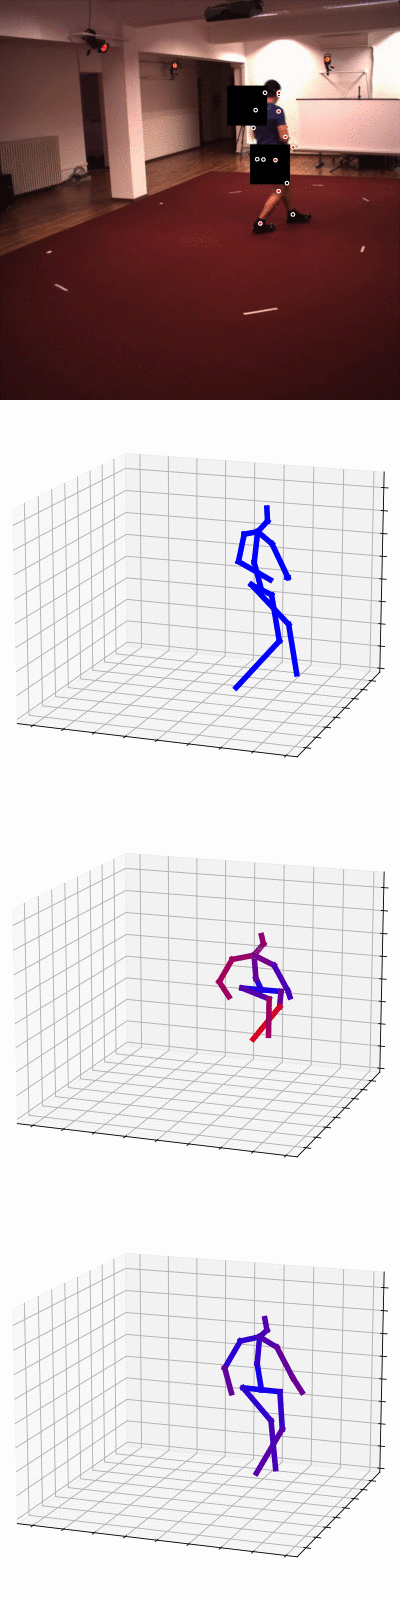}};
        \draw (\w * 1, \h * \r)node[inner sep=0]  {\includegraphics[width=1.57cm]{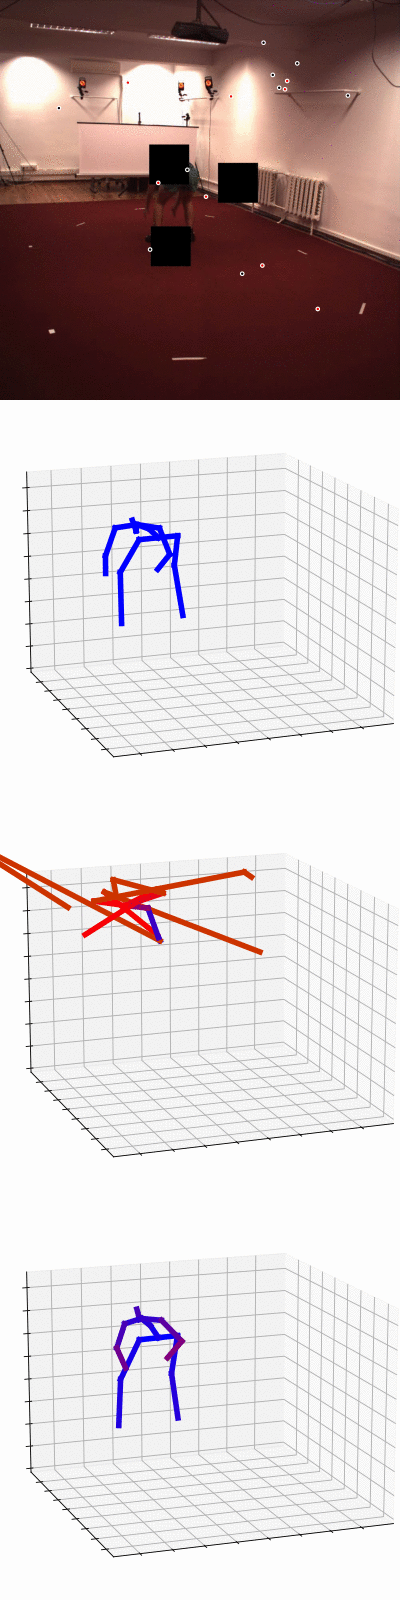}};
        \draw (\w * 2, \h * \r) node[inner sep=0] {\includegraphics[width=1.57cm]{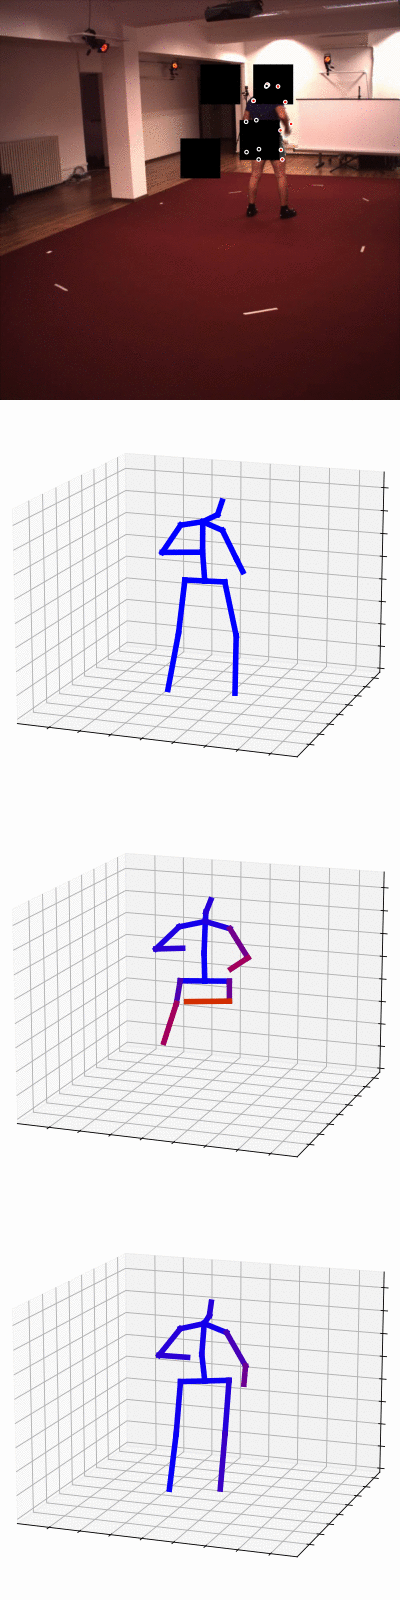}};
        \draw (\w * 3 ,\h * \r) node[inner sep=0] {\includegraphics[width=1.57cm]{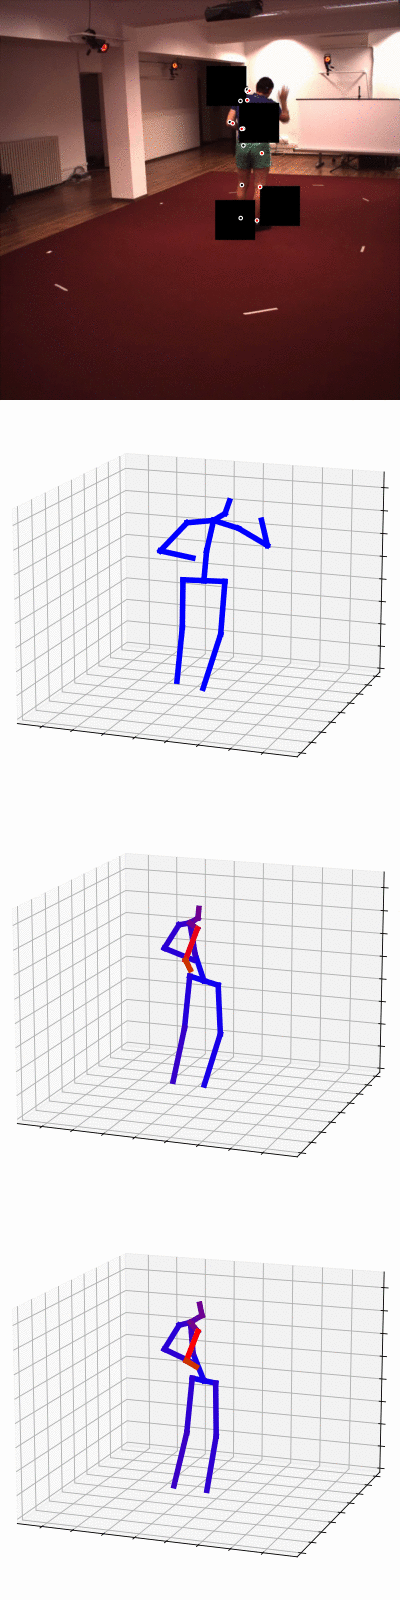}};
        \draw (\w * 4, \h * \r) node[inner sep=0] {\includegraphics[width=1.57cm]{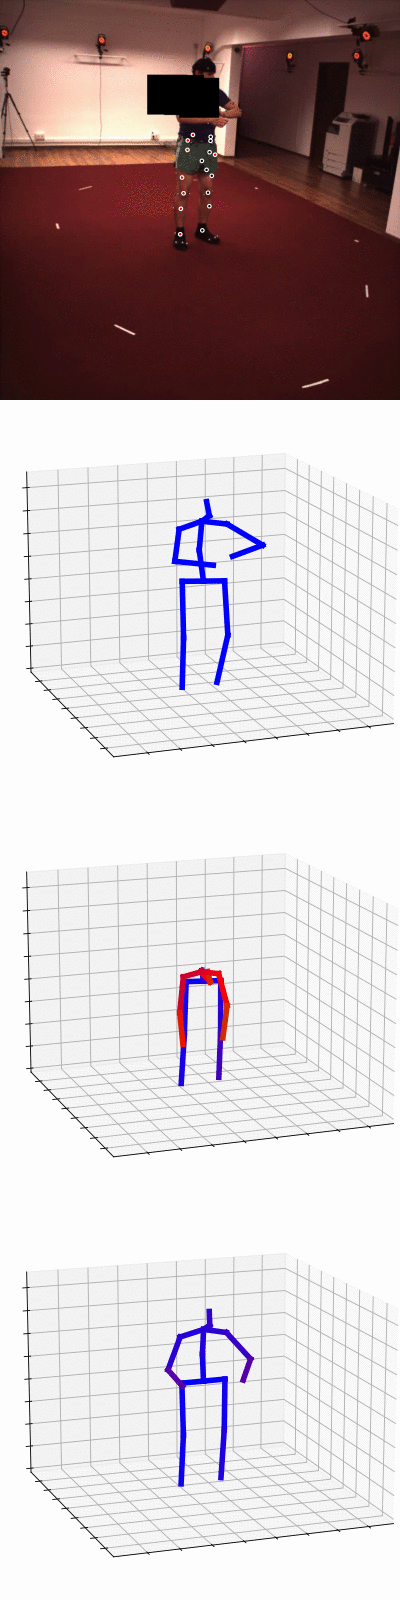}};
        \draw (\w * 5, \h * \r) node[inner sep=0] {\includegraphics[width=1.57cm]{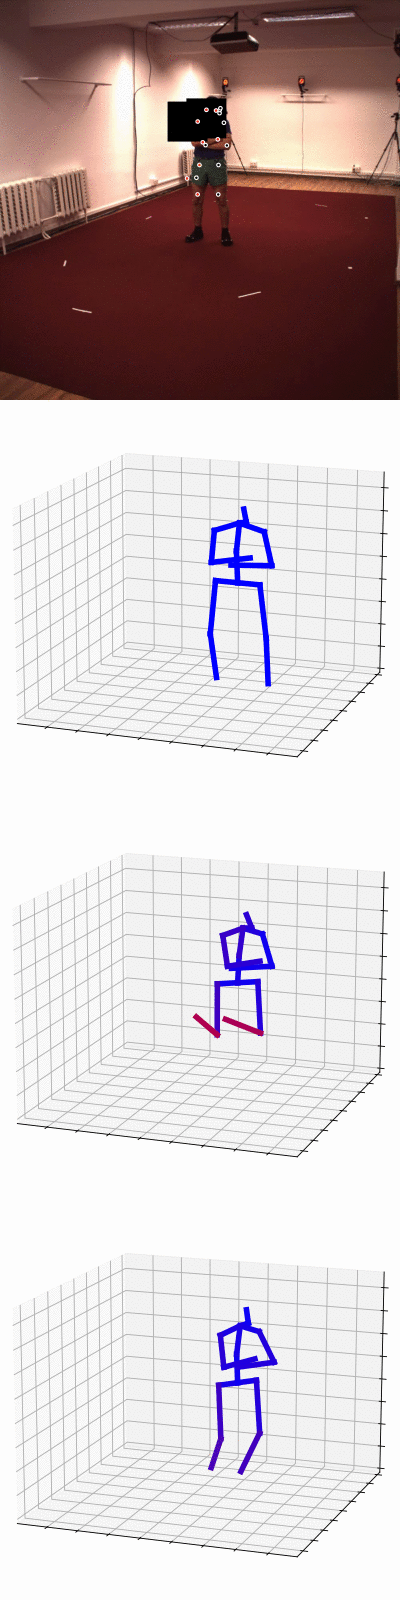}};
        \draw (\w * 6, \h * \r) node[inner sep=0] {\includegraphics[width=1.57cm]{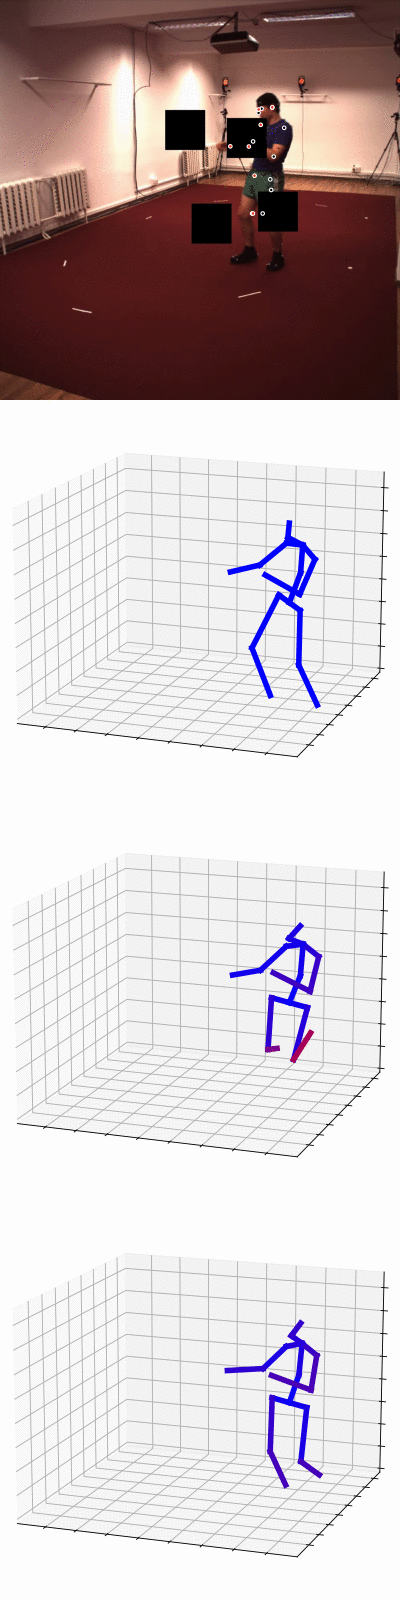}};
        \draw (\w * 7, \h * \r) node[inner sep=0] {\includegraphics[width=1.57cm]{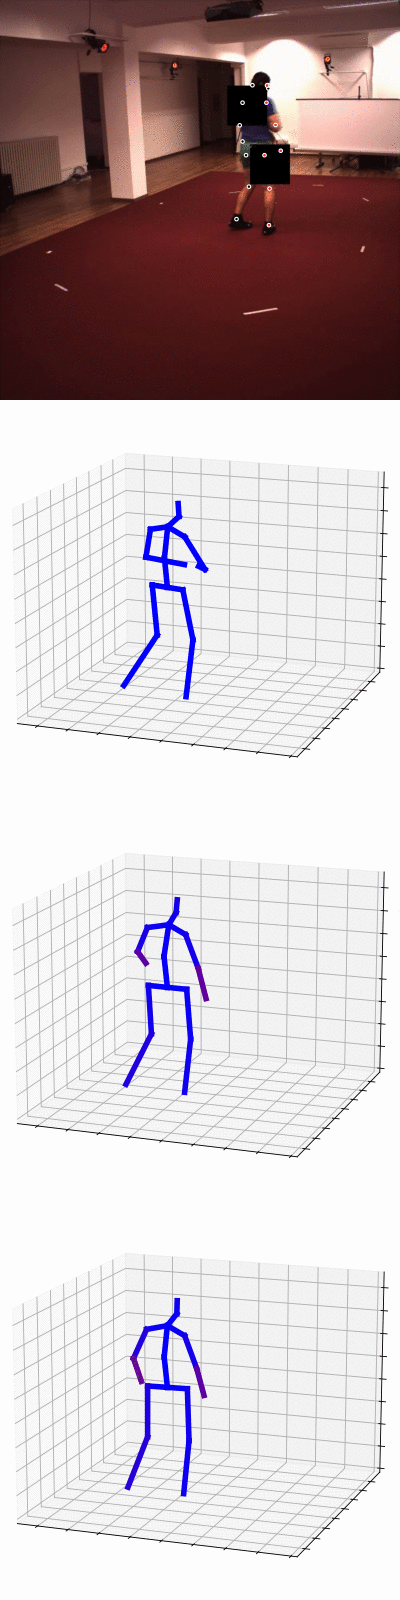}};
        \draw (\w * 8, \h * \r) node[inner sep=0] {\includegraphics[width=1.57cm]{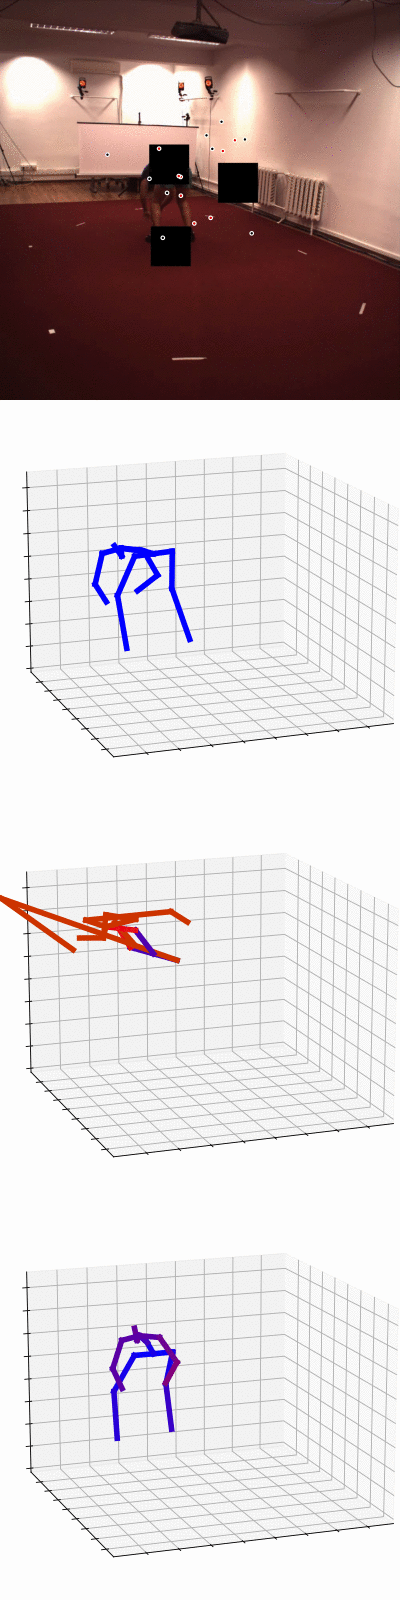}};
        \draw (\w * 9, \h * \r) node[inner sep=0] {\includegraphics[width=1.57cm]{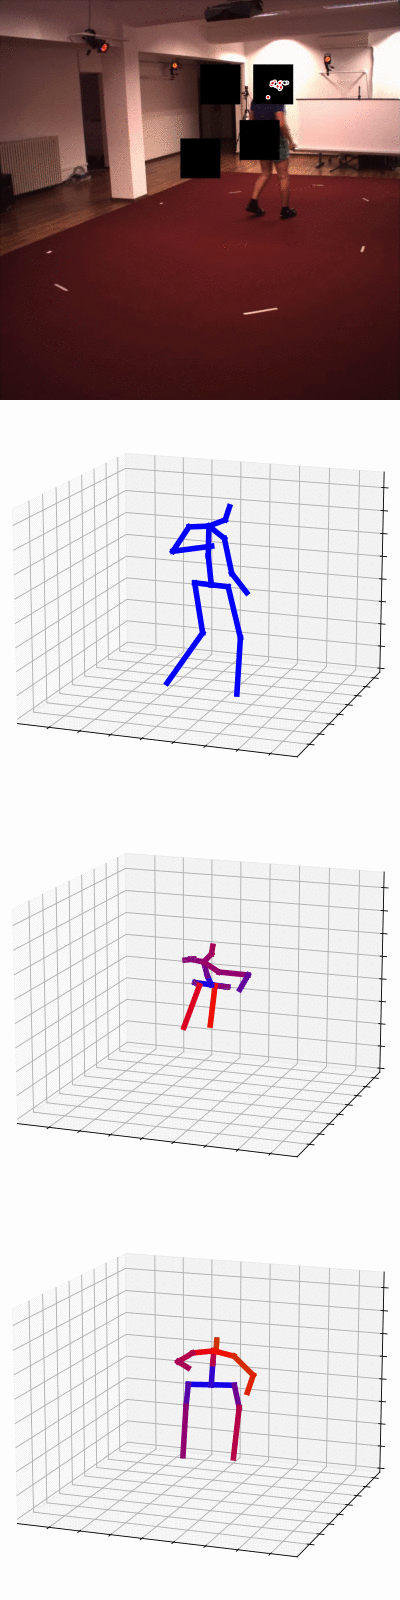}};
        
        \def \r{1} 
        \node at (-1.5, \h * \r - \u * 4 , 0) [below, rotate=90] {\footnotesize{VP3D + }};
        \node at (-1.25, \h * \r - \u * 4, 0) [below, rotate=90] {\footnotesize{TAGN}};
        \node at (-1.375, \h * \r - \u * 1.5, 0) [below, rotate=90] {\footnotesize{VP3D}};
        \node at (-1.375, \h * \r + \u * 1.2, 0) [below, rotate=90] {\footnotesize{GT}};
        \node at (-1.375, \h * \r + \u * 4,  0) [below, rotate=90] {\footnotesize{Frame}};
        \draw (\w * 0, \h * \r) node[inner sep=0] {\includegraphics[width=1.57cm]{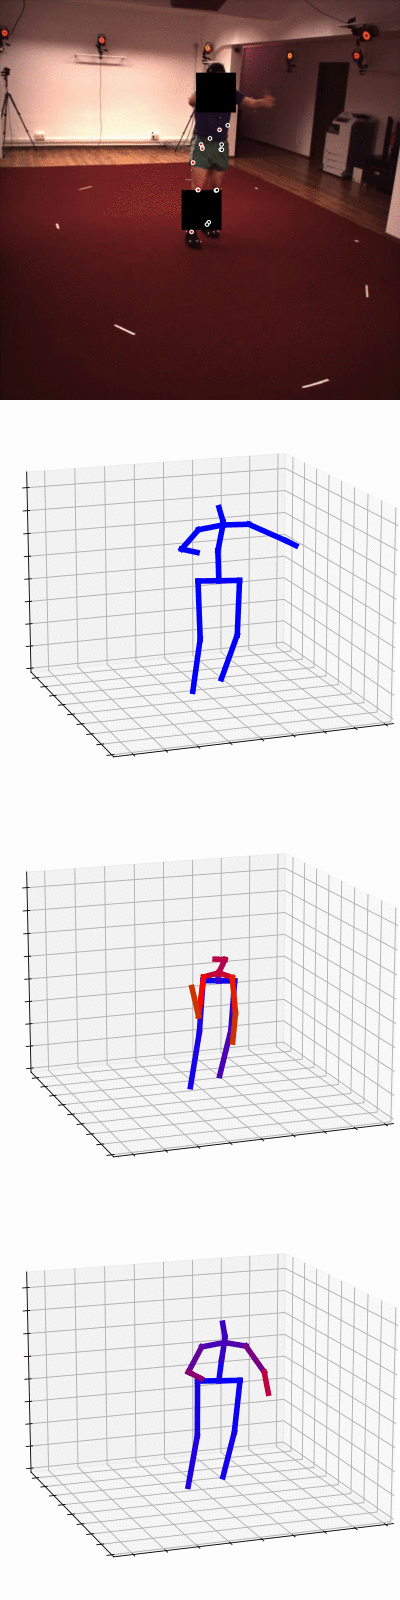}};
        \draw (\w * 1, \h * \r)node[inner sep=0]  {\includegraphics[width=1.57cm]{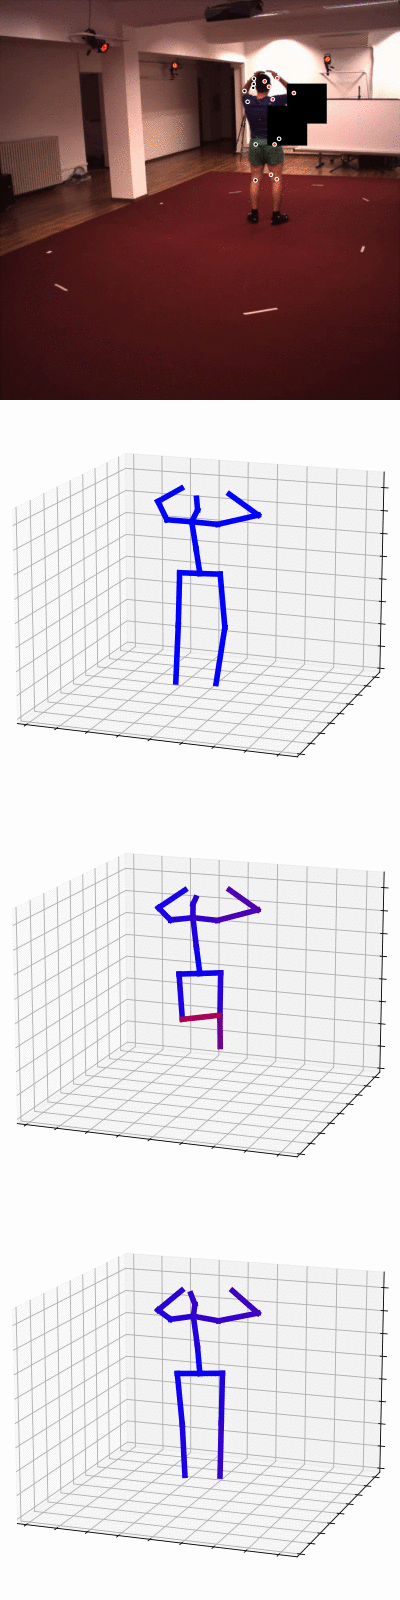}};
        \draw (\w * 2, \h * \r) node[inner sep=0] {\includegraphics[width=1.57cm]{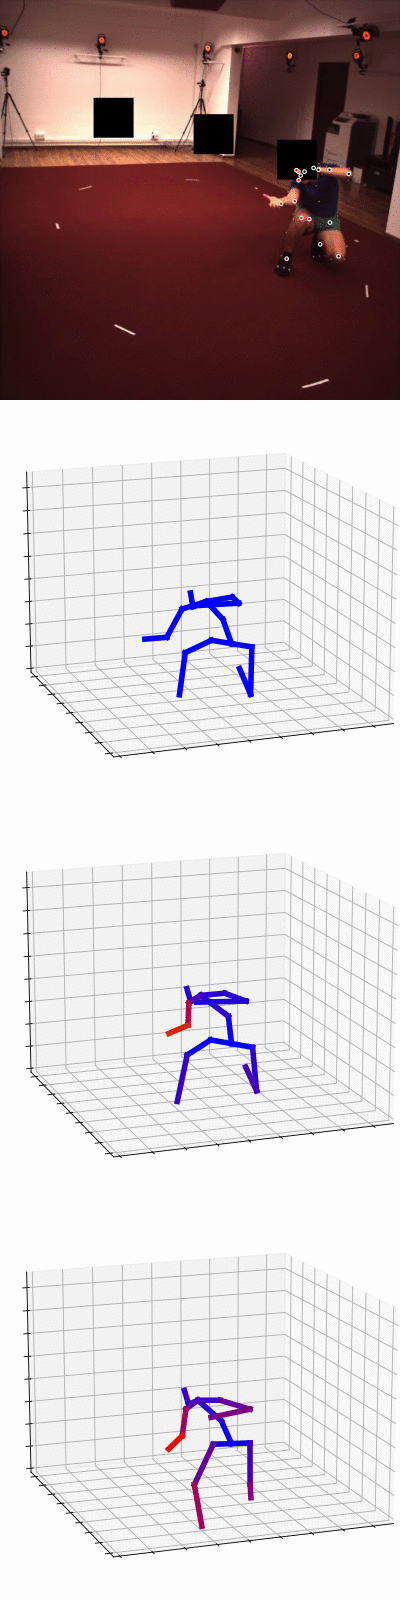}};
        \draw (\w * 3 ,\h * \r) node[inner sep=0] {\includegraphics[width=1.57cm]{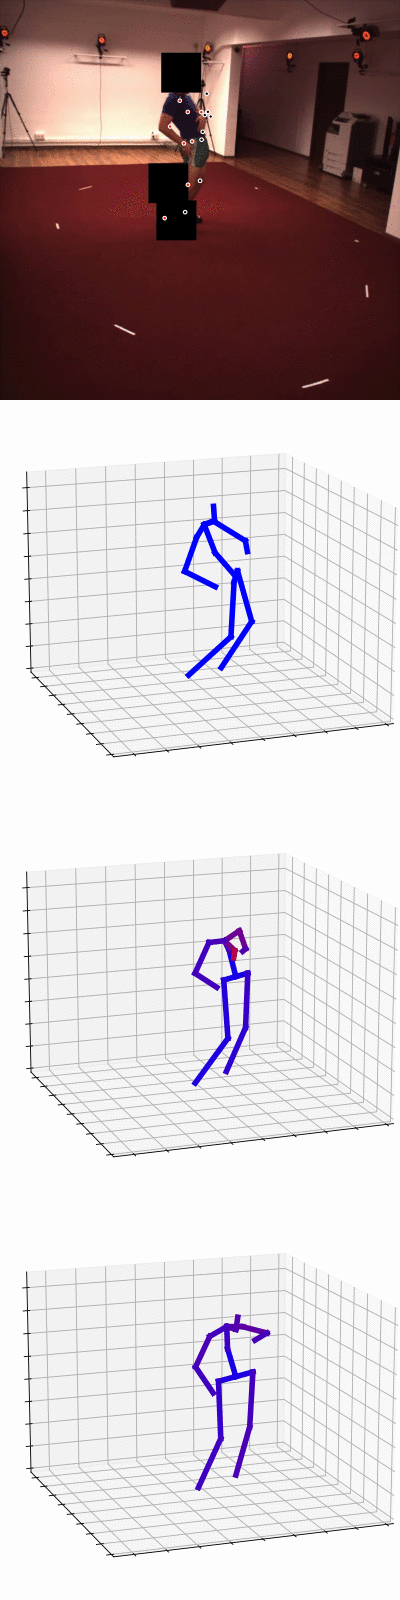}};
        \draw (\w * 4, \h * \r) node[inner sep=0] {\includegraphics[width=1.57cm]{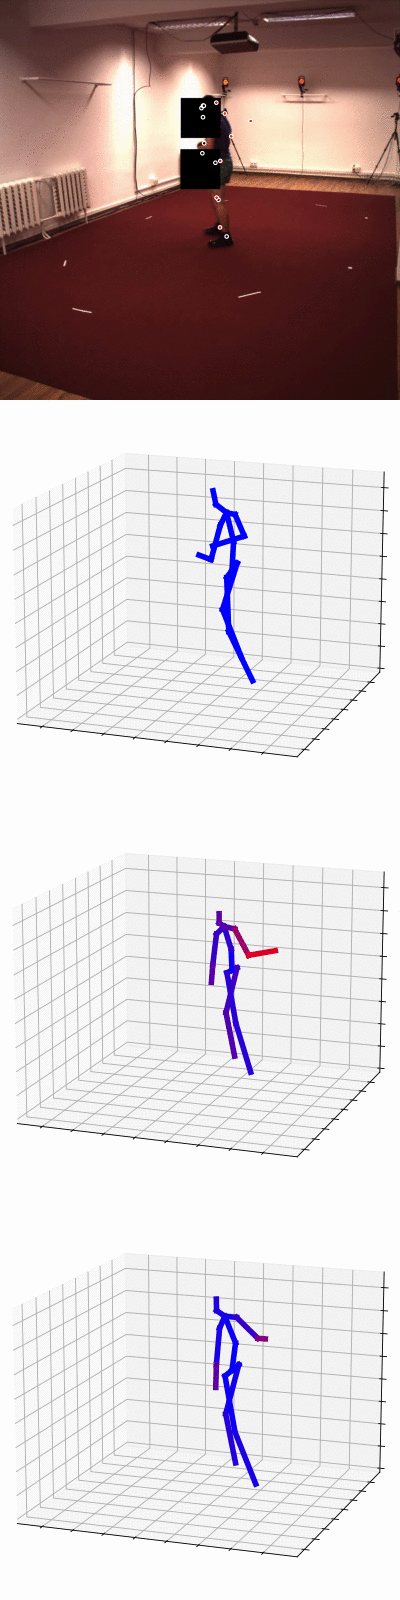}};
        \draw (\w * 5, \h * \r) node[inner sep=0] {\includegraphics[width=1.57cm]{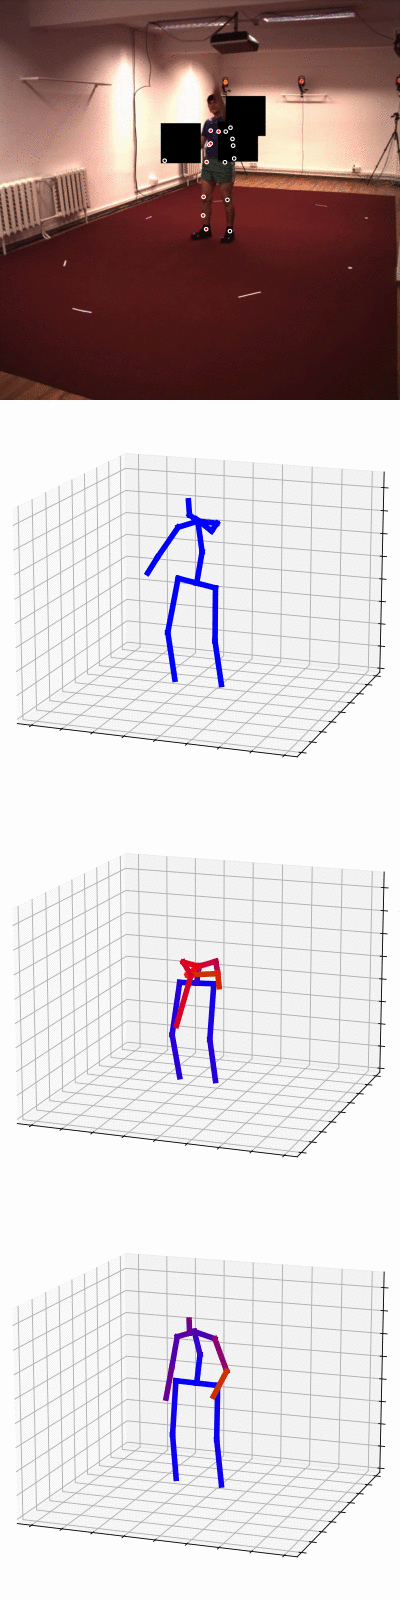}};
        \draw (\w * 6, \h * \r) node[inner sep=0] {\includegraphics[width=1.57cm]{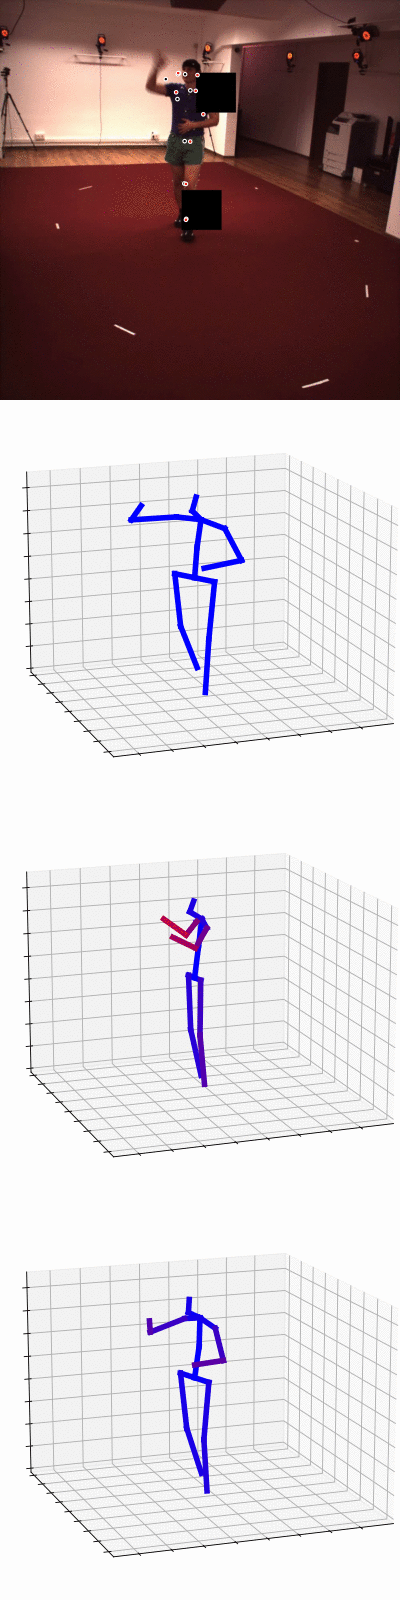}};
        \draw (\w * 7, \h * \r) node[inner sep=0] {\includegraphics[width=1.57cm]{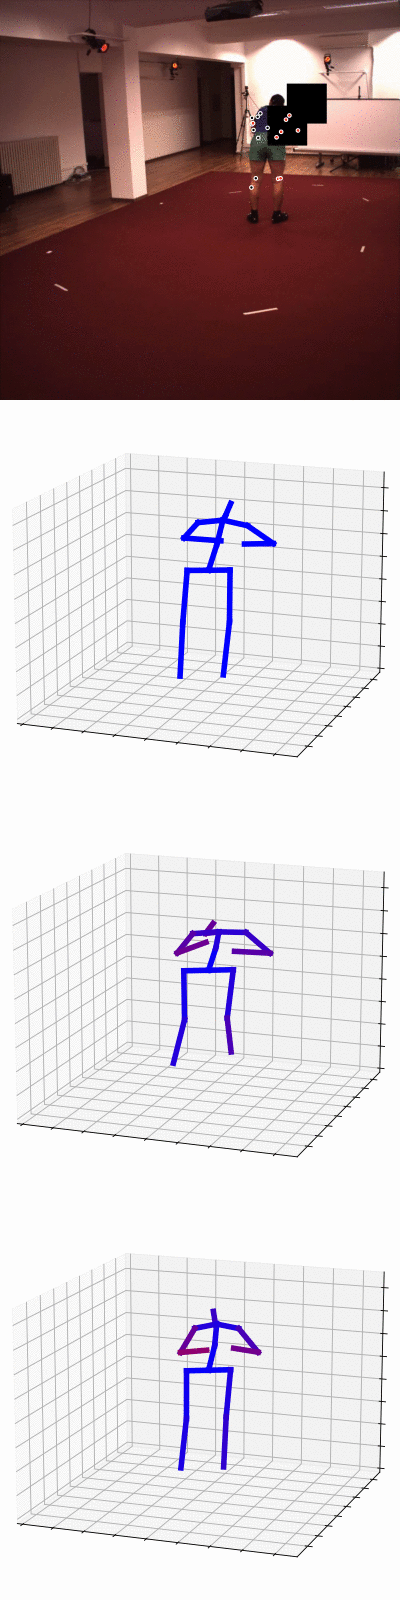}};
        \draw (\w * 8, \h * \r) node[inner sep=0] {\includegraphics[width=1.57cm]{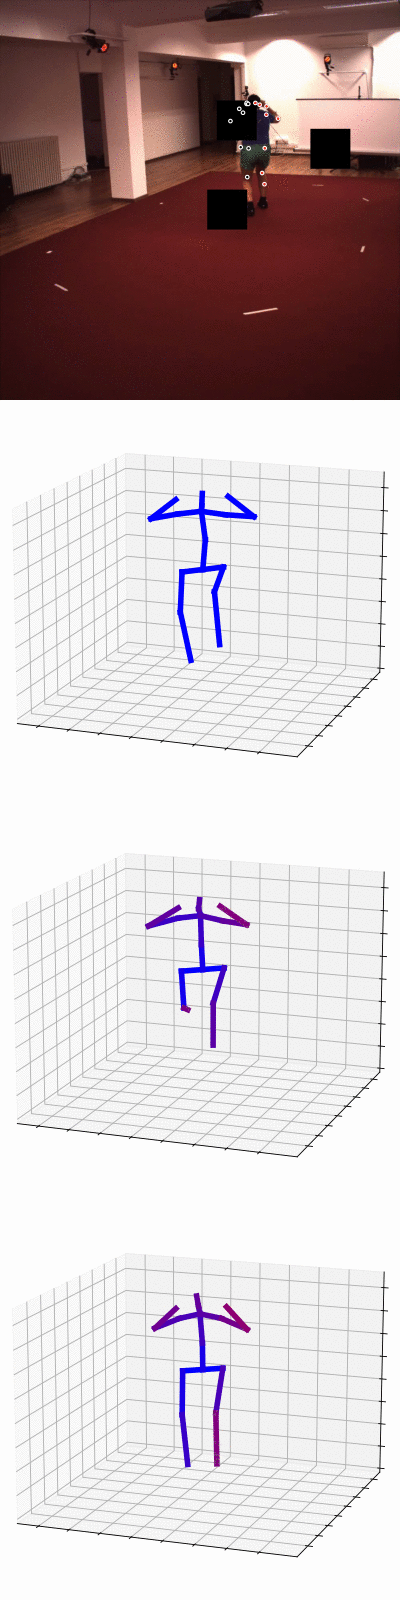}};
        \draw (\w * 9, \h * \r) node[inner sep=0] {\includegraphics[width=1.57cm]{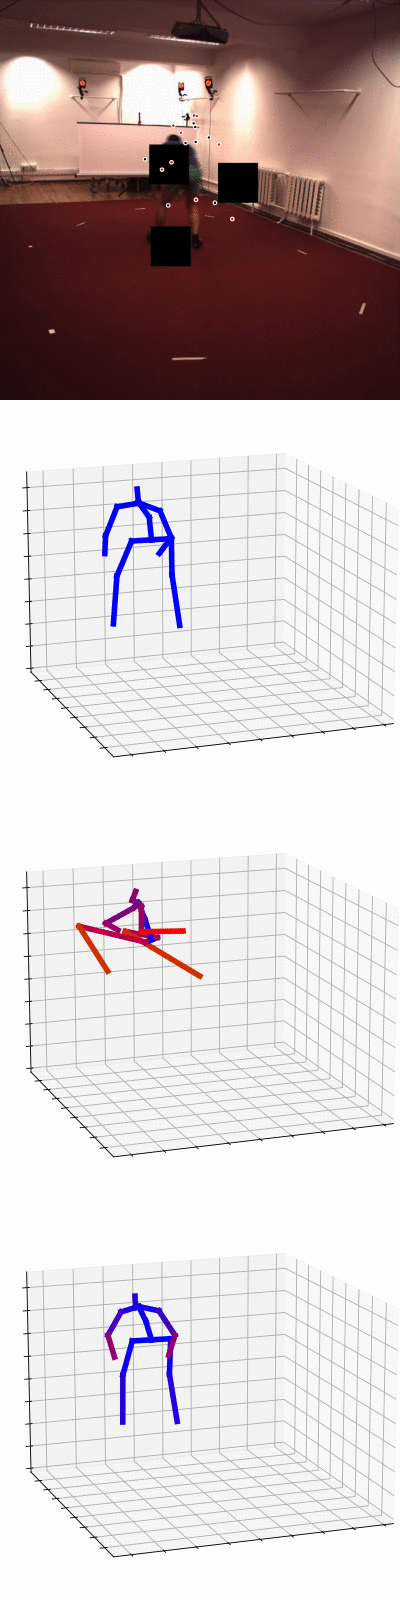}};
        
        \def \r{2}  
        \node at (-1.5, \h * \r - \u * 4 , 0) [below, rotate=90] {\footnotesize{VP3D + }};
        \node at (-1.25, \h * \r - \u * 4, 0) [below, rotate=90] {\footnotesize{TAGN}};
        \node at (-1.375, \h * \r - \u * 1.5, 0) [below, rotate=90] {\footnotesize{VP3D}};
        \node at (-1.375, \h * \r + \u * 1.2, 0) [below, rotate=90] {\footnotesize{GT}};
        \node at (-1.375, \h * \r + \u * 4,  0) [below, rotate=90] {\footnotesize{Frame}};
        \draw (\w * 0, \h * \r) node[inner sep=0] {\includegraphics[width=1.57cm]{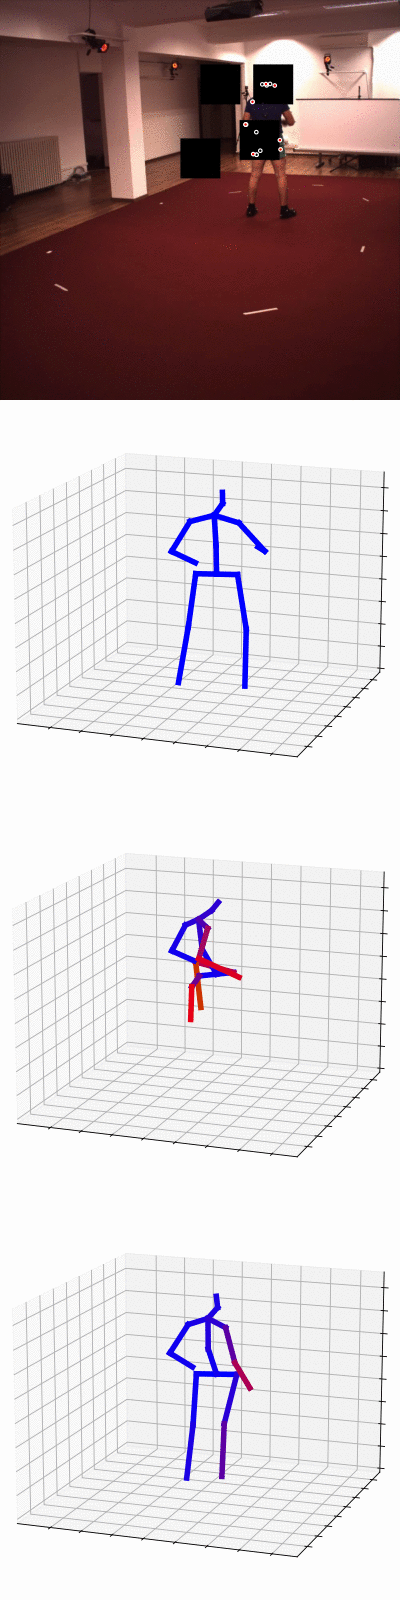}};
        \draw (\w * 1, \h * \r)node[inner sep=0]  {\includegraphics[width=1.57cm]{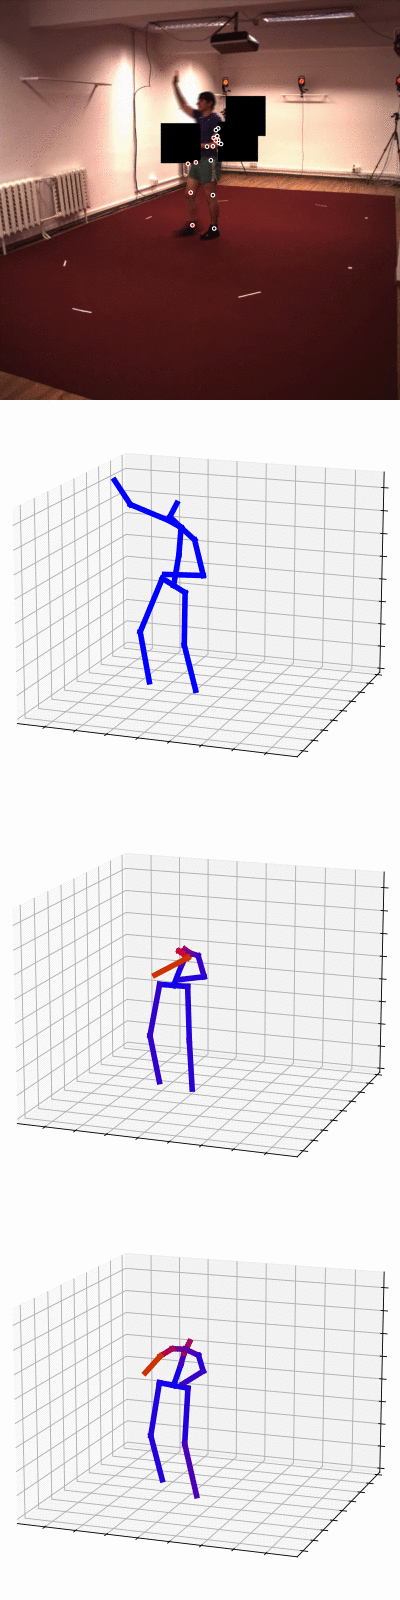}};
        \draw (\w * 2, \h * \r) node[inner sep=0] {\includegraphics[width=1.57cm]{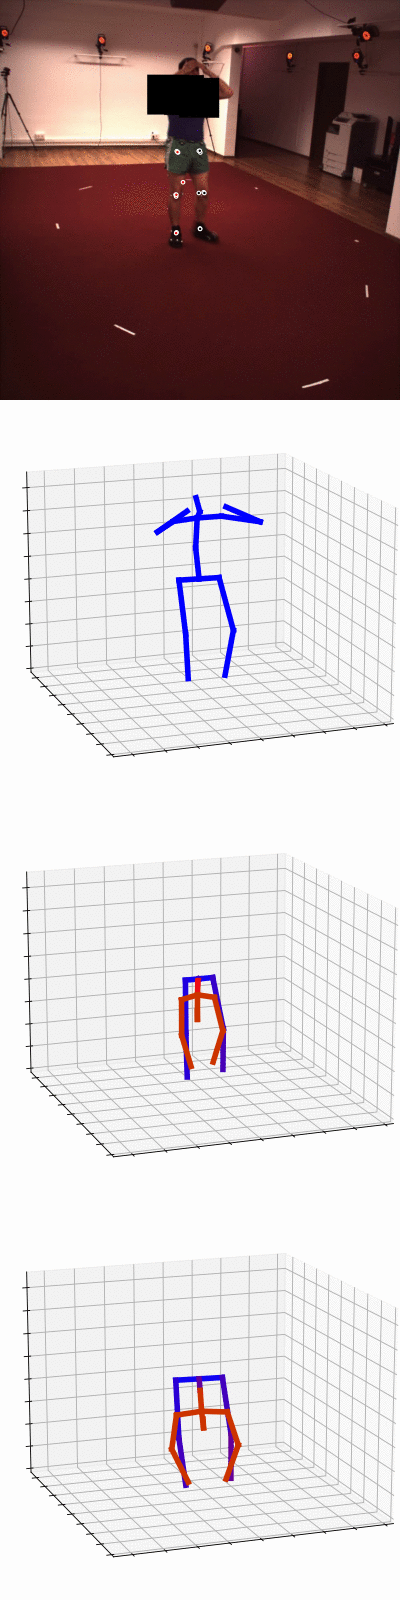}};
        \draw (\w * 3 ,\h * \r) node[inner sep=0] {\includegraphics[width=1.57cm]{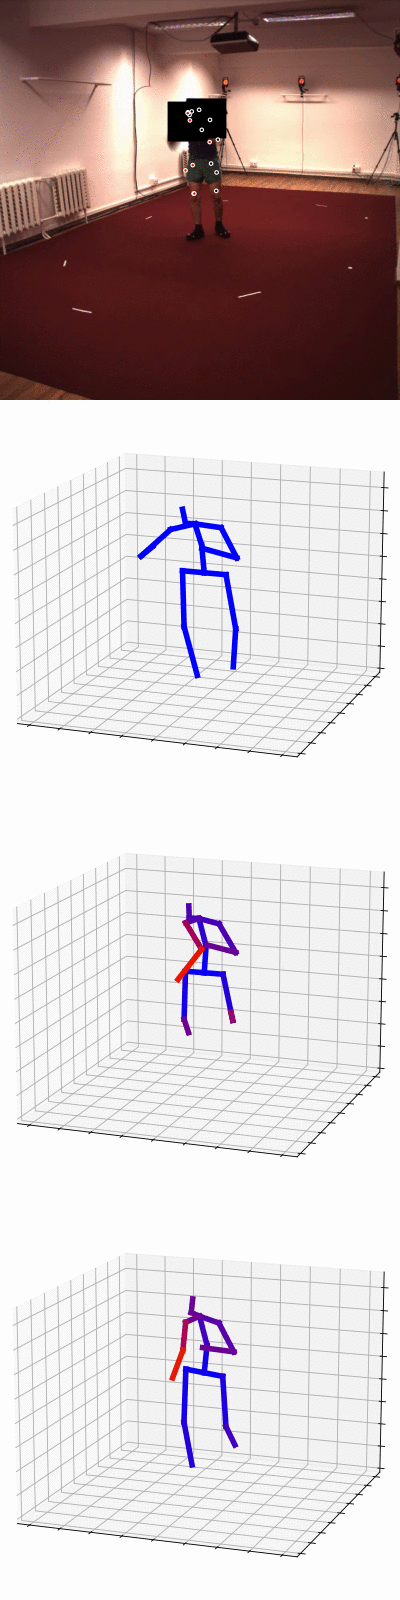}};
        \draw (\w * 4, \h * \r) node[inner sep=0] {\includegraphics[width=1.57cm]{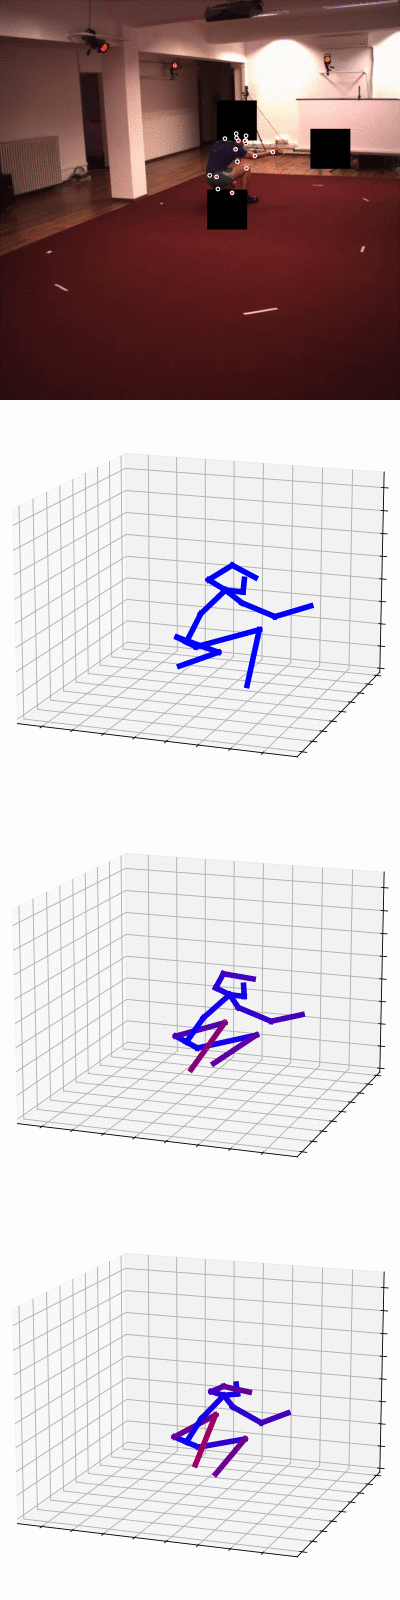}};
        \draw (\w * 5, \h * \r) node[inner sep=0] {\includegraphics[width=1.57cm]{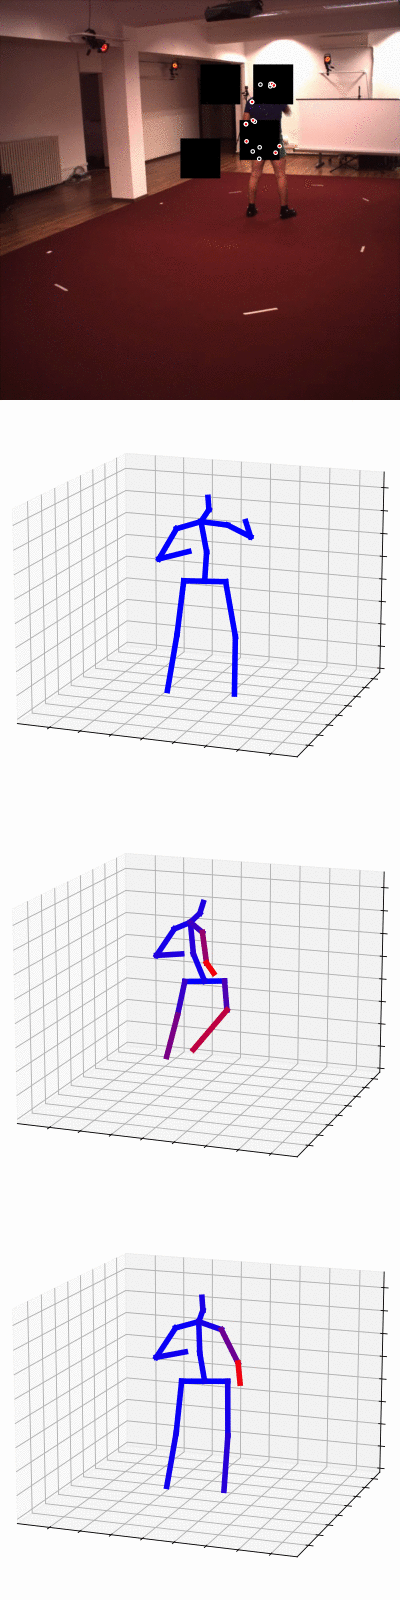}};
        \draw (\w * 6, \h * \r) node[inner sep=0] {\includegraphics[width=1.57cm]{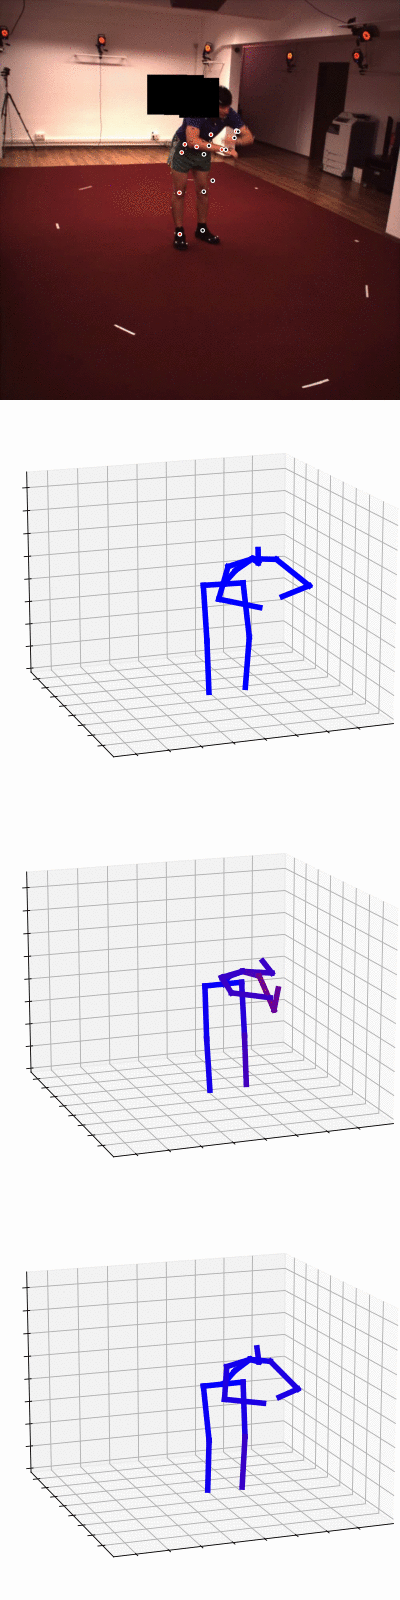}};
        \draw (\w * 7, \h * \r) node[inner sep=0] {\includegraphics[width=1.57cm]{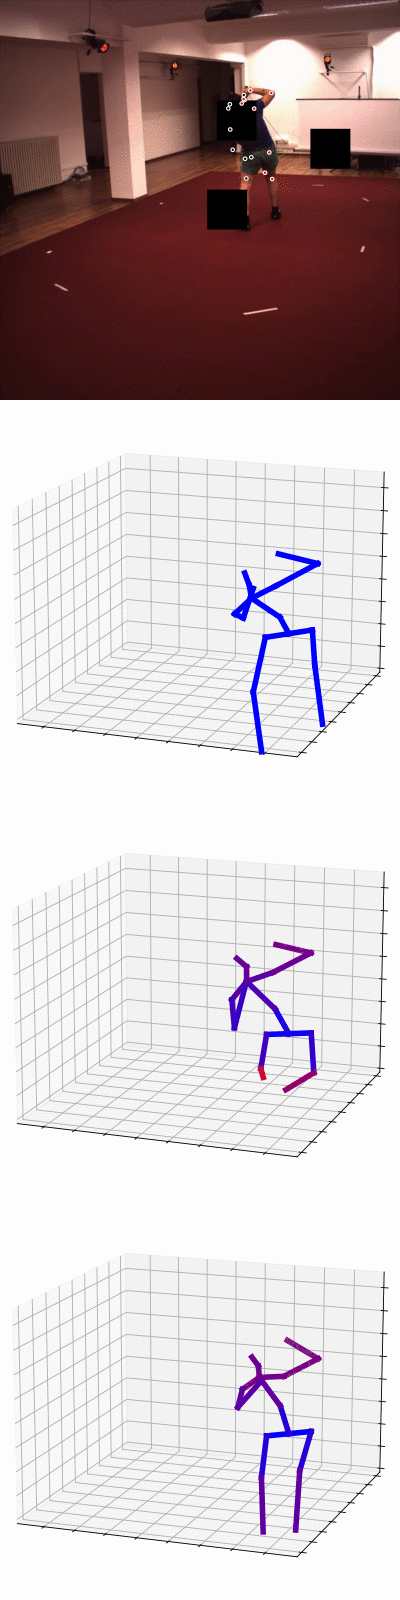}};
        \draw (\w * 8, \h * \r) node[inner sep=0] {\includegraphics[width=1.57cm]{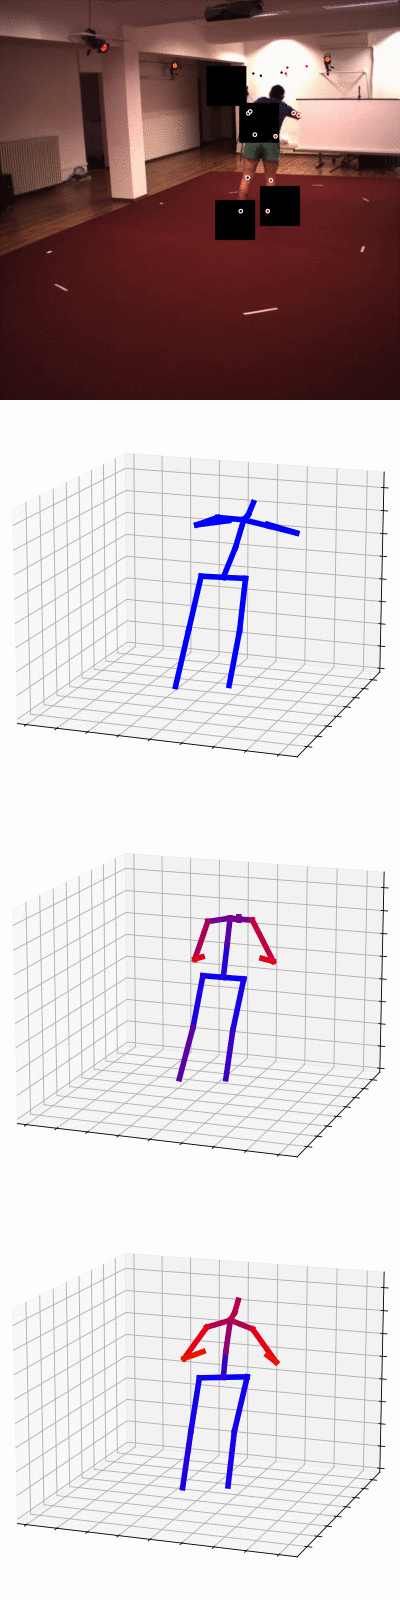}};
        \draw (\w * 9, \h * \r) node[inner sep=0] {\includegraphics[width=1.57cm]{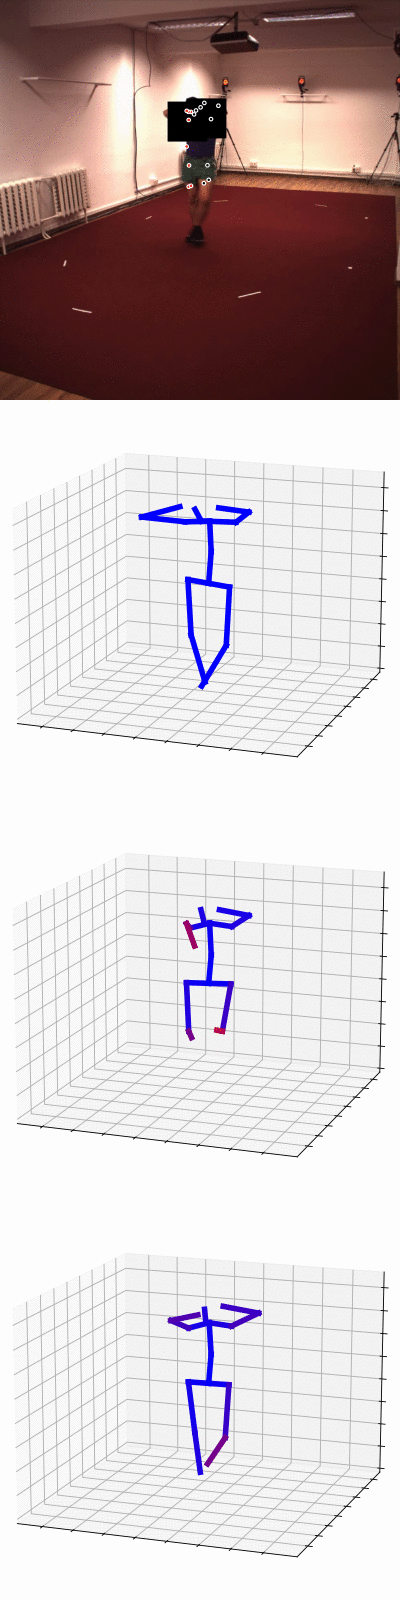}};

        \end{tikzpicture}
    \vspace*{-0.5\baselineskip}
    \caption{Qualitative comparison of VP3D+TAGN ($\sigma=0.3, p=k=50\%$) versus VP3D, on H36M-C dataset (with guided-patch erasing corruption). The bone color leading to a joint turns \textcolor{red}{red} when its MPJPE increases.}
    \vspace*{-\baselineskip}
    \label{fig:supp-tagn-qualitative}
\end{figure*}

Lastly, in Figure~\ref{fig:supp-tagn-qualitative}, we visualize additional qualitative comparisons between VP3D\cite{pavllo2019_videopose3d} and VP3D \cite{pavllo2019_videopose3d} + TAGN models, both trained on the original Human3.6M \cite{h36m_pami} dataset.
