# Supplementary material for: Improving the Robustness of 3D Human Pose Estimation: A Benchmark and Learning from Noisy Input
Source: arXiv:2312.06797 source file (2024-04-16)
Supplement: Supplementary file 2 [file frame_viz_supp.tex]

\begin{figure*}[t!]
    \pgfplotsset{every x tick label/.append style={font=\tiny, yshift=0.5ex}}
    \pgfplotsset{every y tick label/.append style={font=\tiny, xshift=0.5ex}}
    \centering
    
        \hspace{-10pt}
        \begin{tikzpicture}
        \def \h{6.5}
        \def \u{0.6}
        \def \w{1.65}

        \def \r{0} 
        \node at (-1.5,\u * -4 , \h * \r) [below, rotate=90] {\footnotesize{VP3D + }};
        \node at (-1.25, \u * -4,\h * \r) [below, rotate=90] {\footnotesize{TAGN}};
        \node at (-1.375, \u * -1.5, \h * \r) [below, rotate=90] {\footnotesize{VP3D}};
        \node at (-1.375, \u * 1.2,  \h * \r) [below, rotate=90] {\footnotesize{GT}};
        \node at (-1.375, \u * 4,  \h * \r) [below, rotate=90] {\footnotesize{Frame}};
        \draw (\w * 0, \h * \r) node[inner sep=0] {\includegraphics[width=1.57cm]{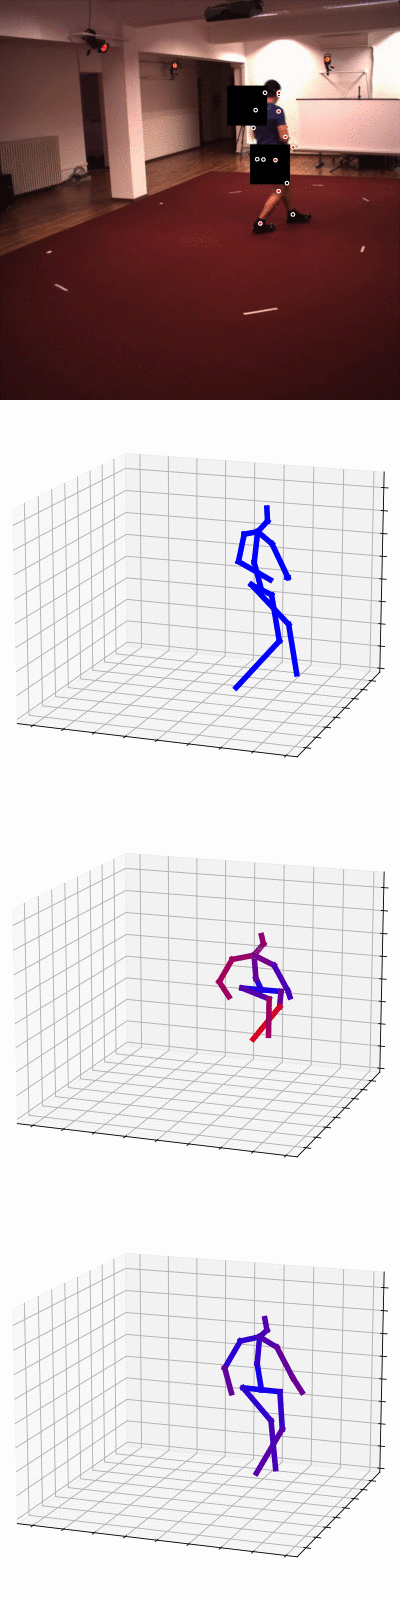}};
        \draw (\w * 1, \h * \r)node[inner sep=0]  {\includegraphics[width=1.57cm]{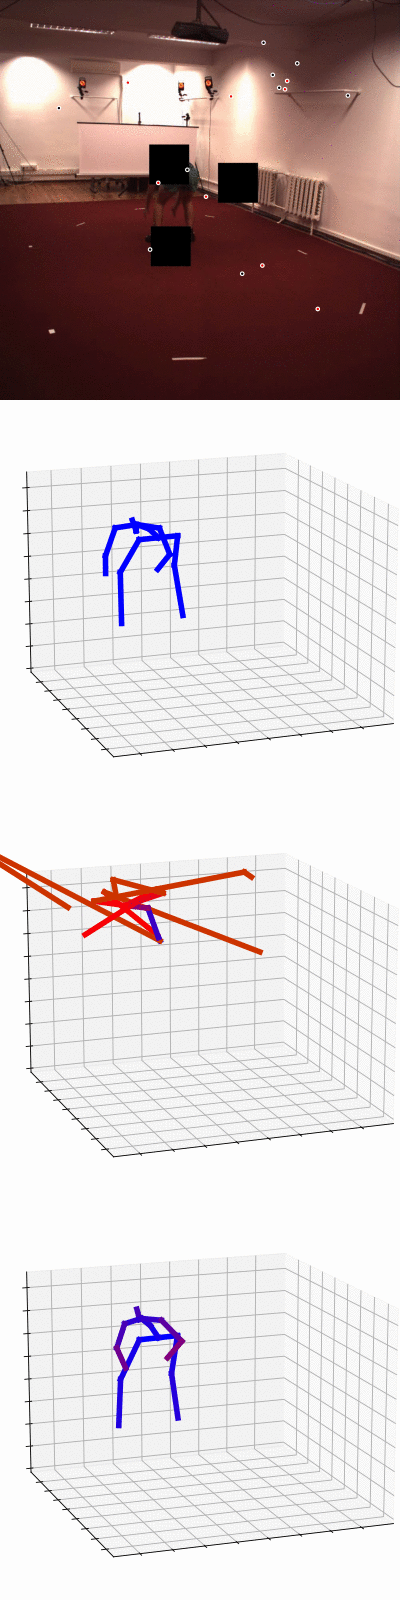}};
        \draw (\w * 2, \h * \r) node[inner sep=0] {\includegraphics[width=1.57cm]{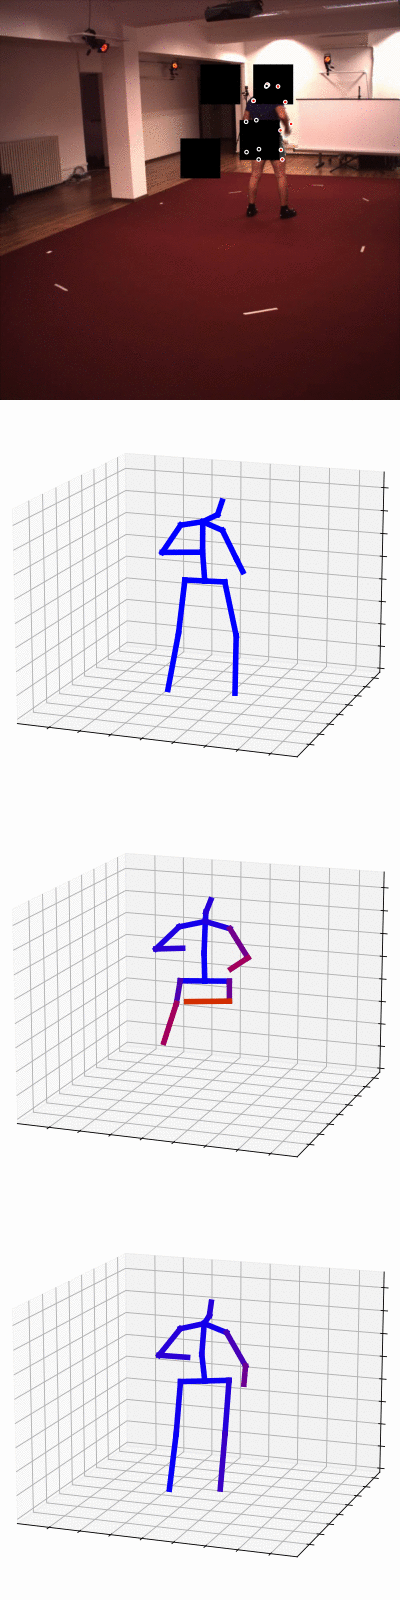}};
        \draw (\w * 3 ,\h * \r) node[inner sep=0] {\includegraphics[width=1.57cm]{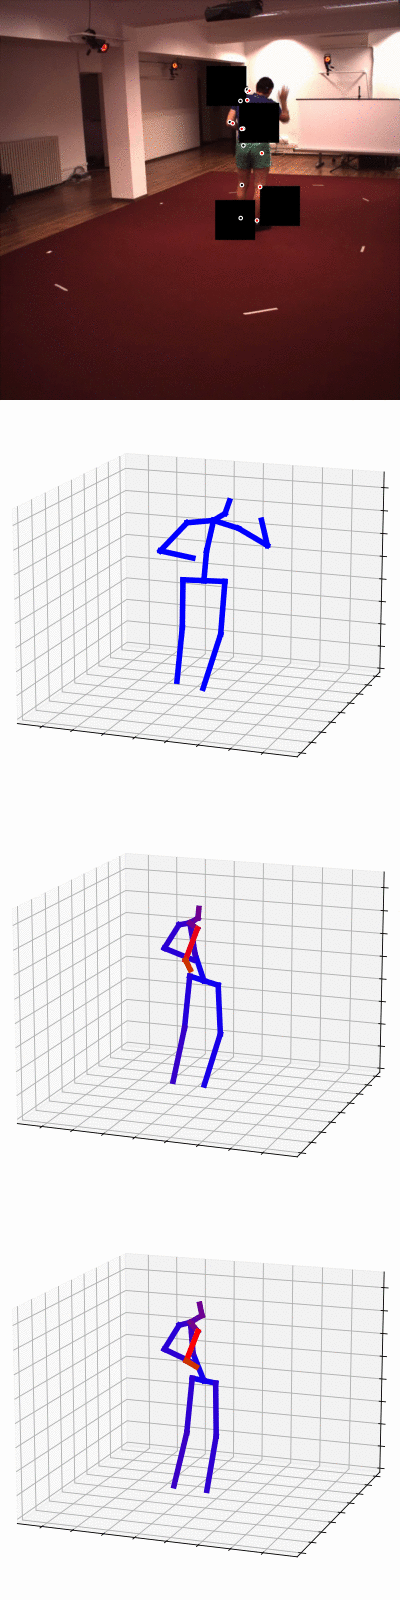}};
        \draw (\w * 4, \h * \r) node[inner sep=0] {\includegraphics[width=1.57cm]{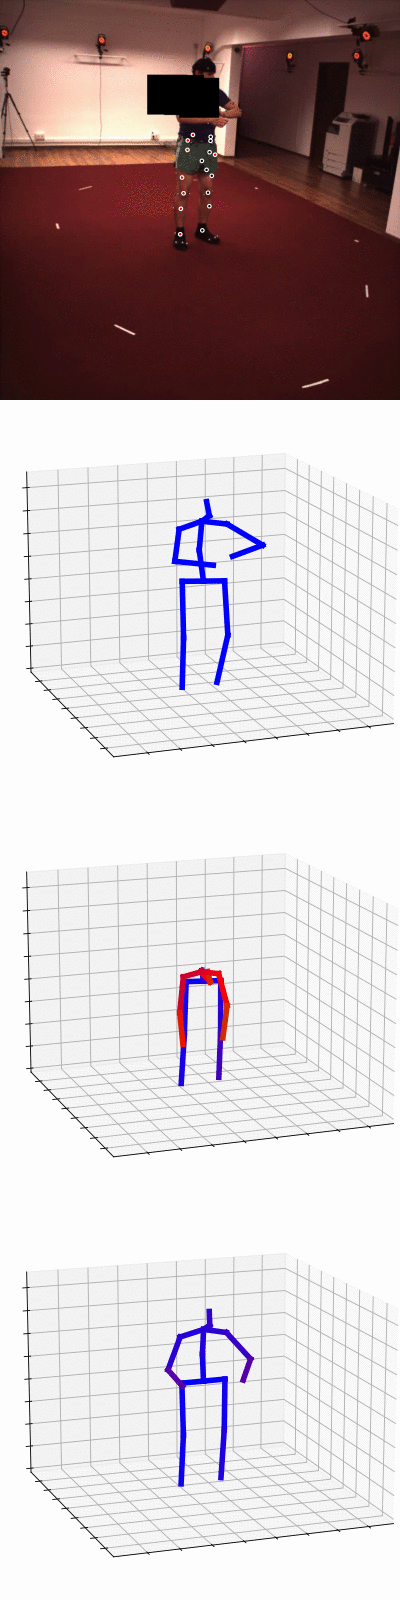}};
        \draw (\w * 5, \h * \r) node[inner sep=0] {\includegraphics[width=1.57cm]{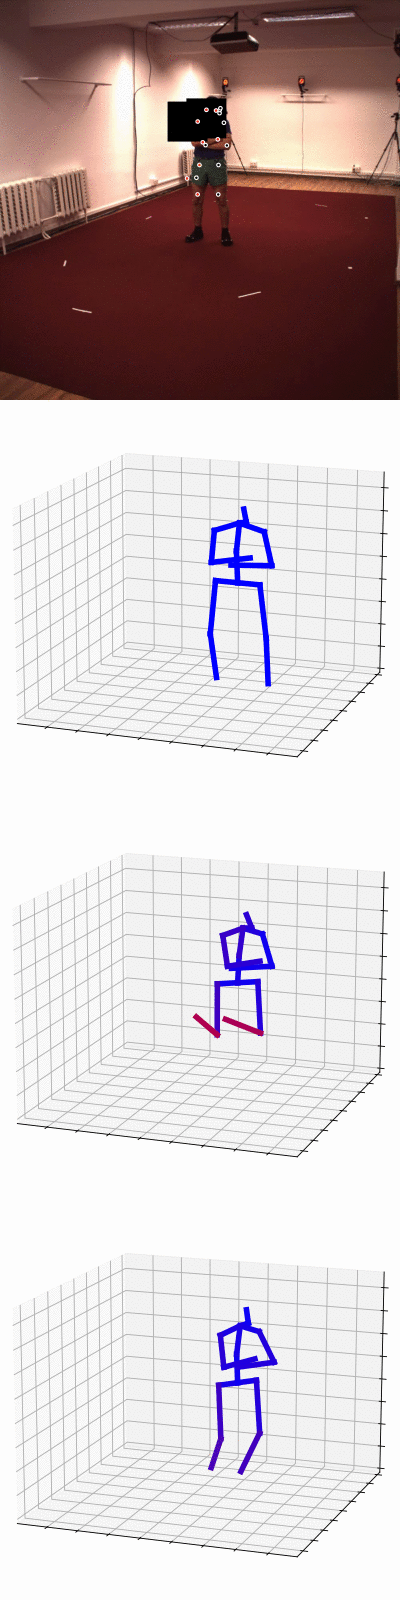}};
        \draw (\w * 6, \h * \r) node[inner sep=0] {\includegraphics[width=1.57cm]{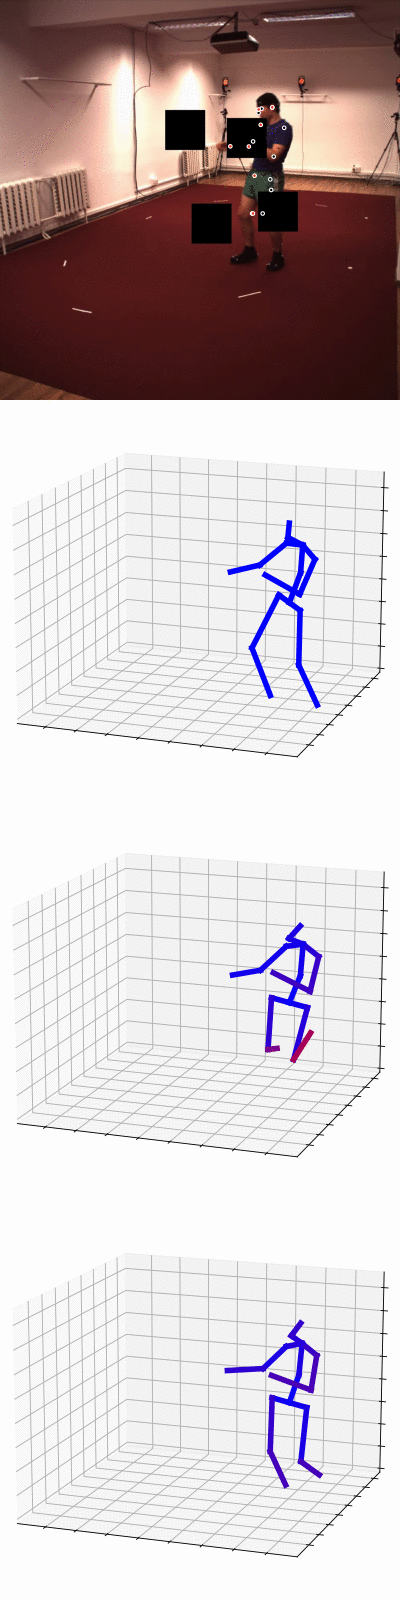}};
        \draw (\w * 7, \h * \r) node[inner sep=0] {\includegraphics[width=1.57cm]{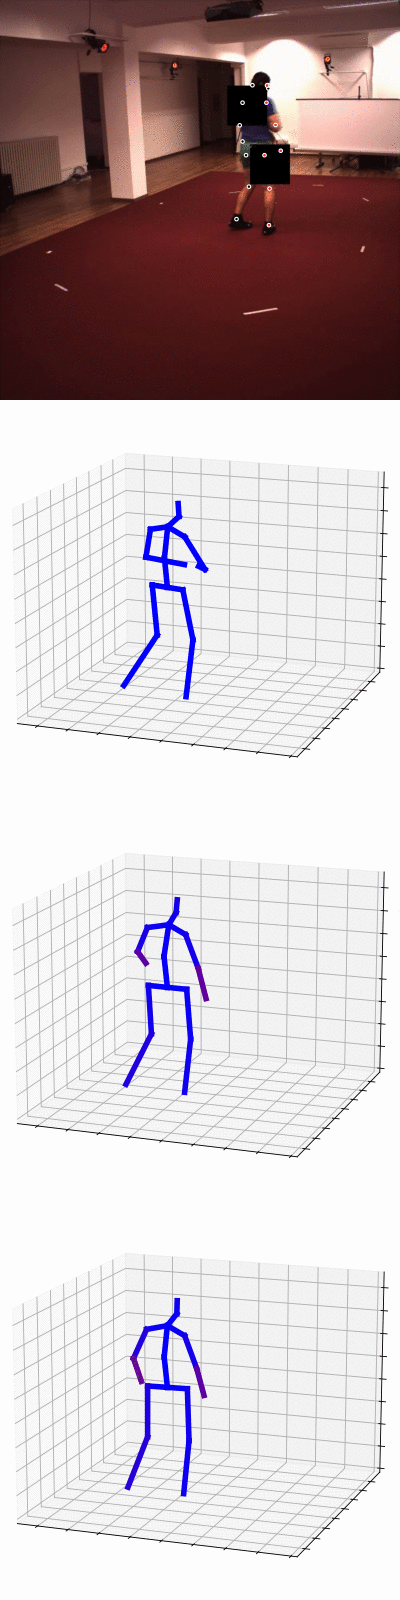}};
        \draw (\w * 8, \h * \r) node[inner sep=0] {\includegraphics[width=1.57cm]{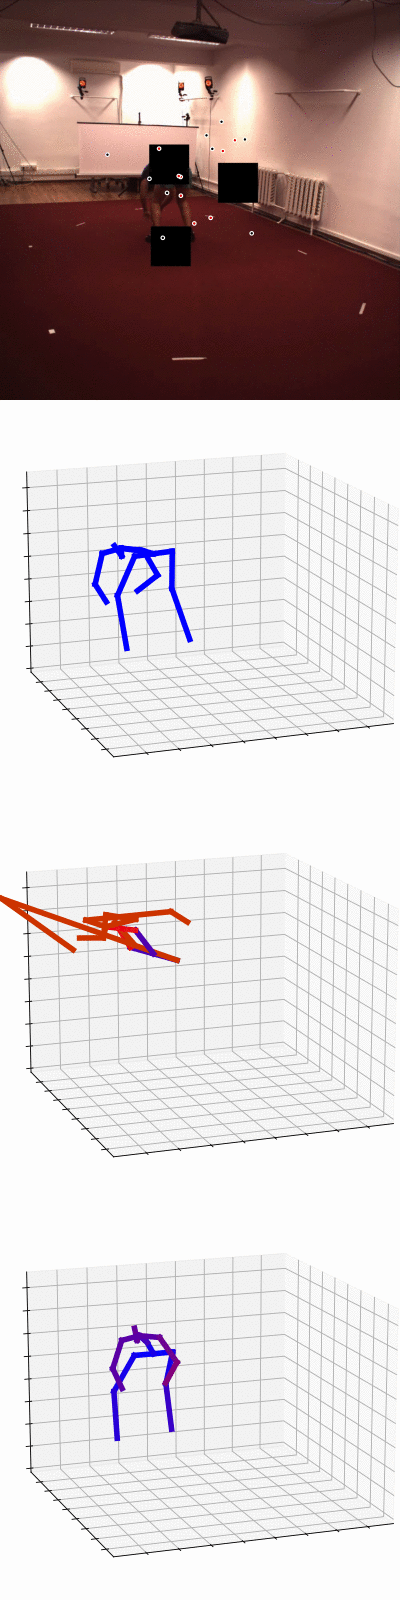}};
        \draw (\w * 9, \h * \r) node[inner sep=0] {\includegraphics[width=1.57cm]{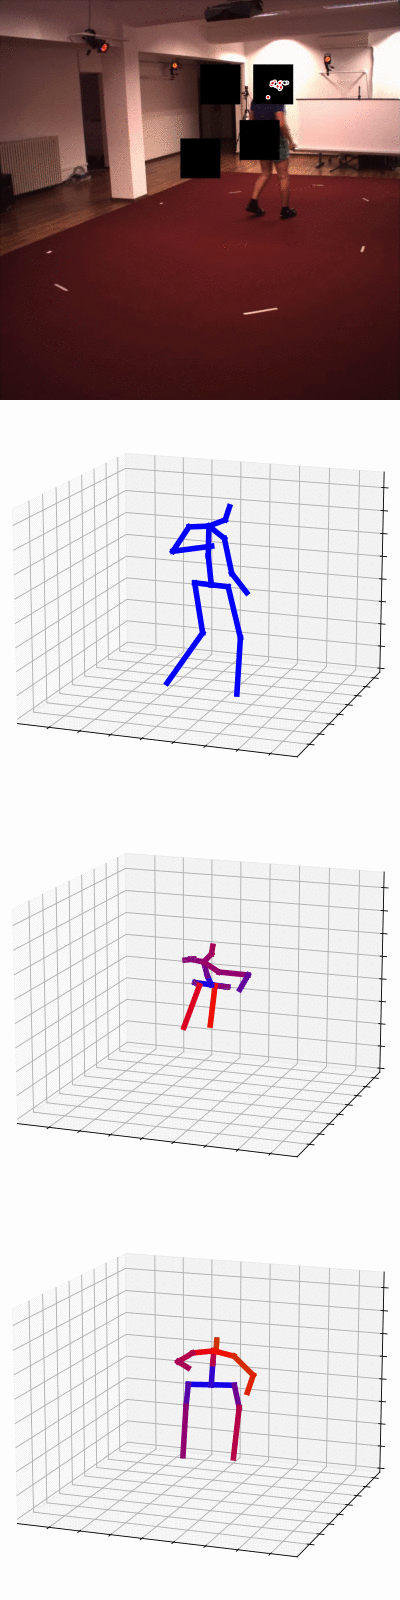}};
        
        \def \r{1} 
        \node at (-1.5, \h * \r - \u * 4 , 0) [below, rotate=90] {\footnotesize{VP3D + }};
        \node at (-1.25, \h * \r - \u * 4, 0) [below, rotate=90] {\footnotesize{TAGN}};
        \node at (-1.375, \h * \r - \u * 1.5, 0) [below, rotate=90] {\footnotesize{VP3D}};
        \node at (-1.375, \h * \r + \u * 1.2, 0) [below, rotate=90] {\footnotesize{GT}};
        \node at (-1.375, \h * \r + \u * 4,  0) [below, rotate=90] {\footnotesize{Frame}};
        \draw (\w * 0, \h * \r) node[inner sep=0] {\includegraphics[width=1.57cm]{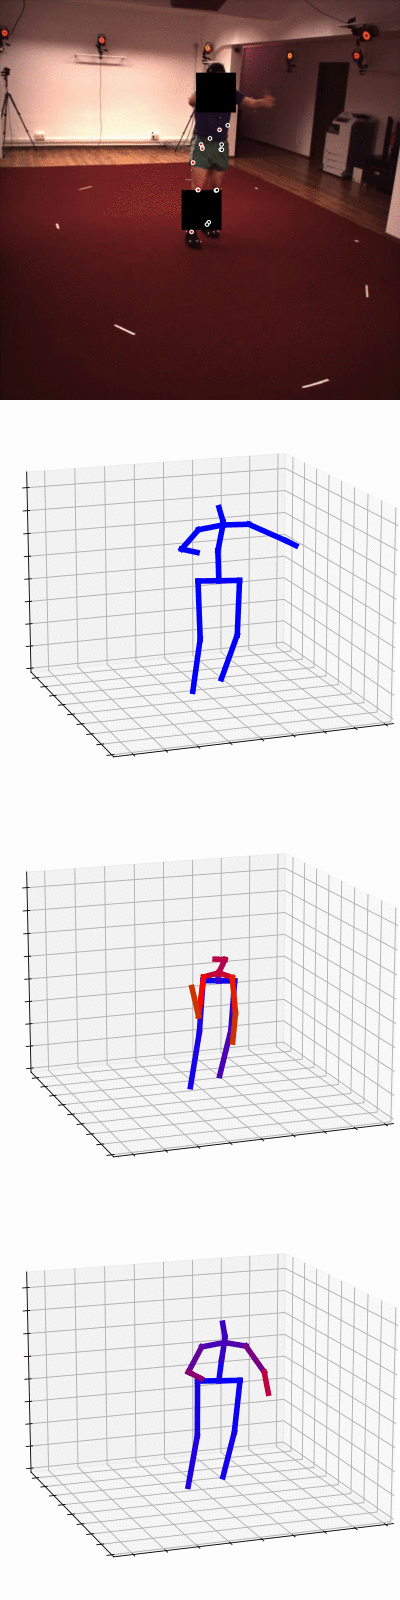}};
        \draw (\w * 1, \h * \r)node[inner sep=0]  {\includegraphics[width=1.57cm]{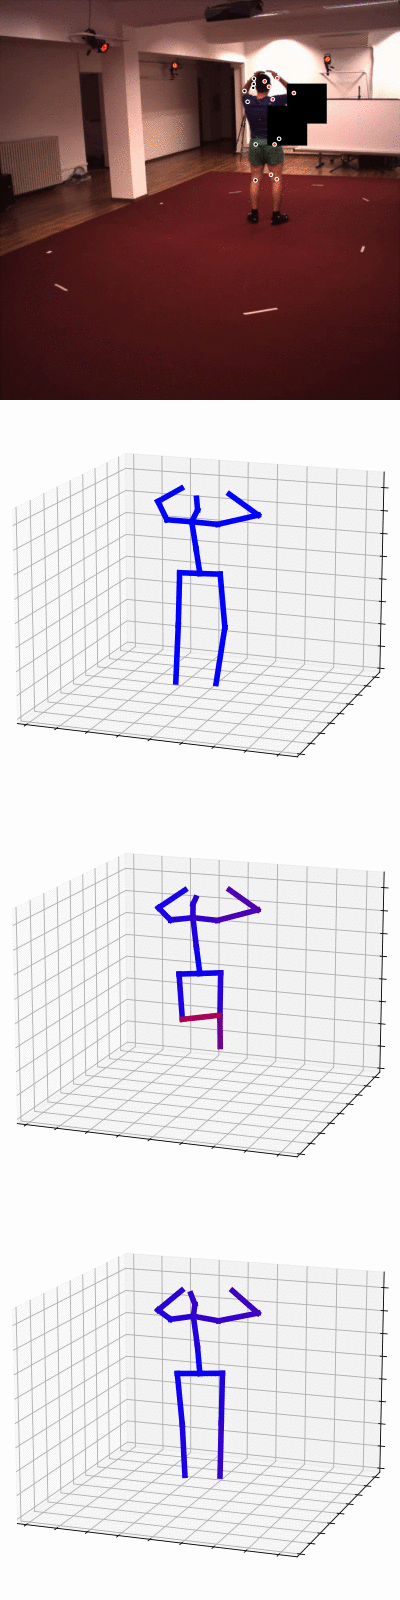}};
        \draw (\w * 2, \h * \r) node[inner sep=0] {\includegraphics[width=1.57cm]{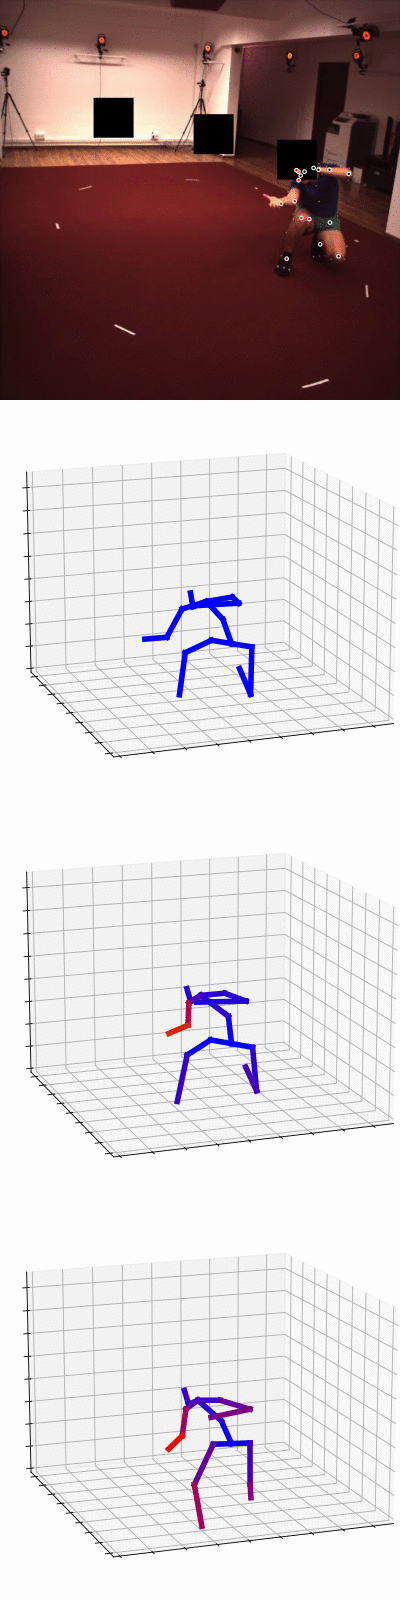}};
        \draw (\w * 3 ,\h * \r) node[inner sep=0] {\includegraphics[width=1.57cm]{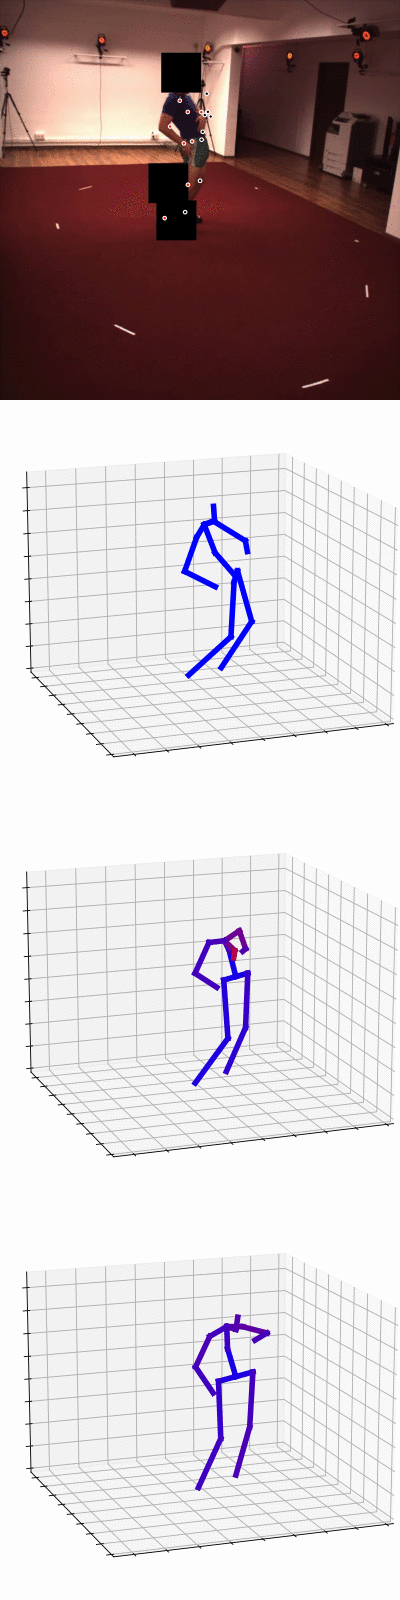}};
        \draw (\w * 4, \h * \r) node[inner sep=0] {\includegraphics[width=1.57cm]{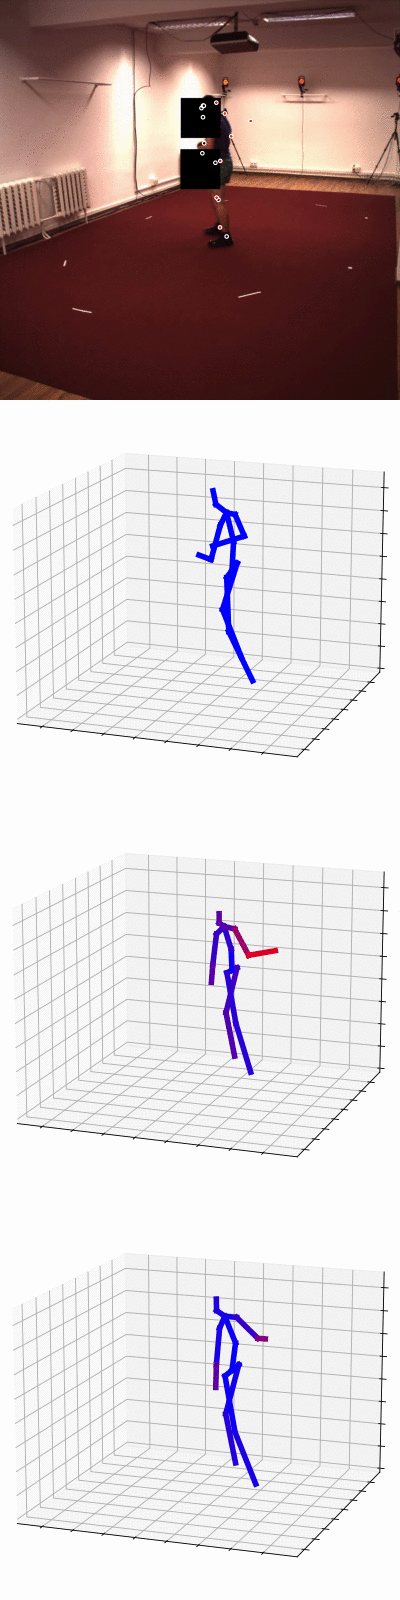}};
        \draw (\w * 5, \h * \r) node[inner sep=0] {\includegraphics[width=1.57cm]{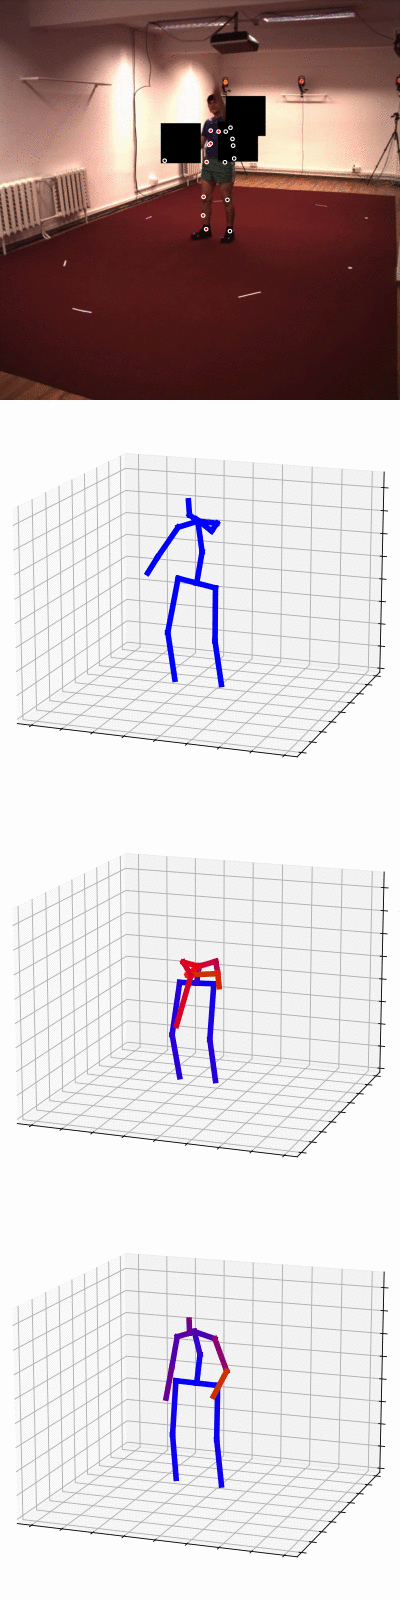}};
        \draw (\w * 6, \h * \r) node[inner sep=0] {\includegraphics[width=1.57cm]{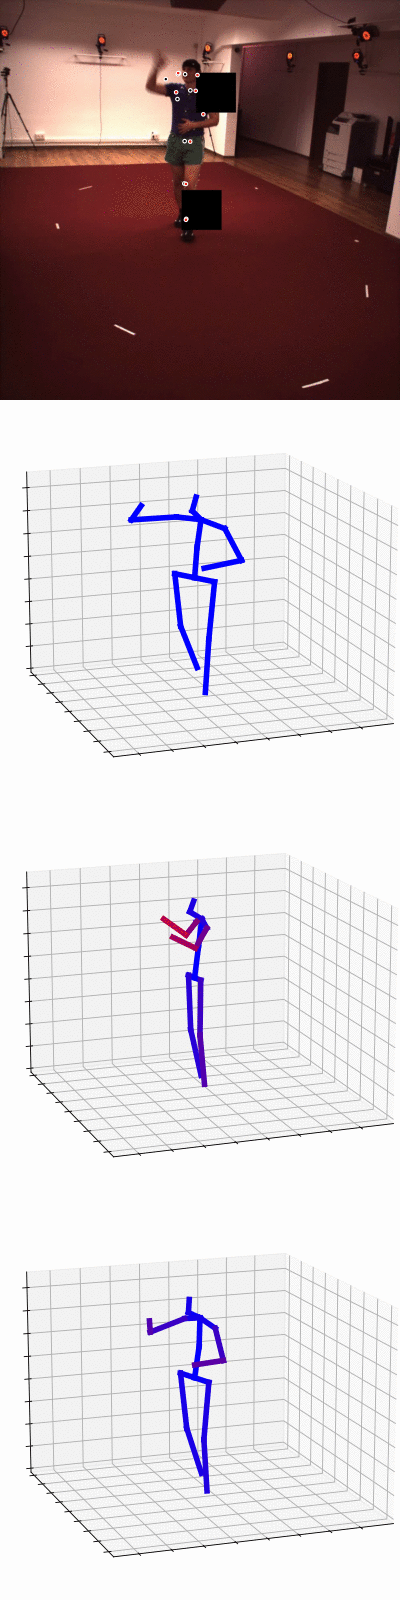}};
        \draw (\w * 7, \h * \r) node[inner sep=0] {\includegraphics[width=1.57cm]{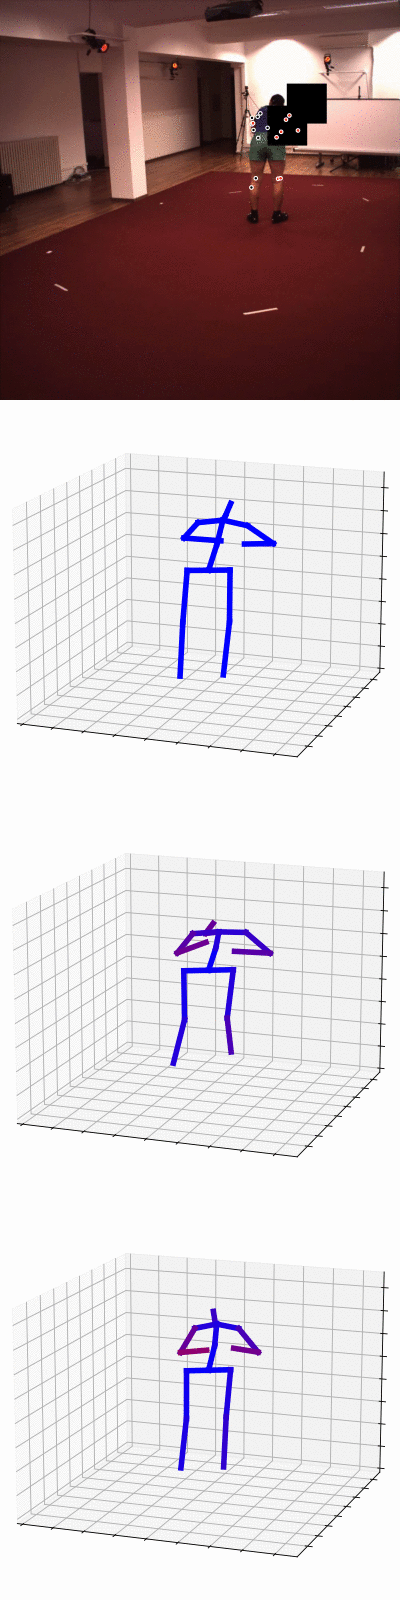}};
        \draw (\w * 8, \h * \r) node[inner sep=0] {\includegraphics[width=1.57cm]{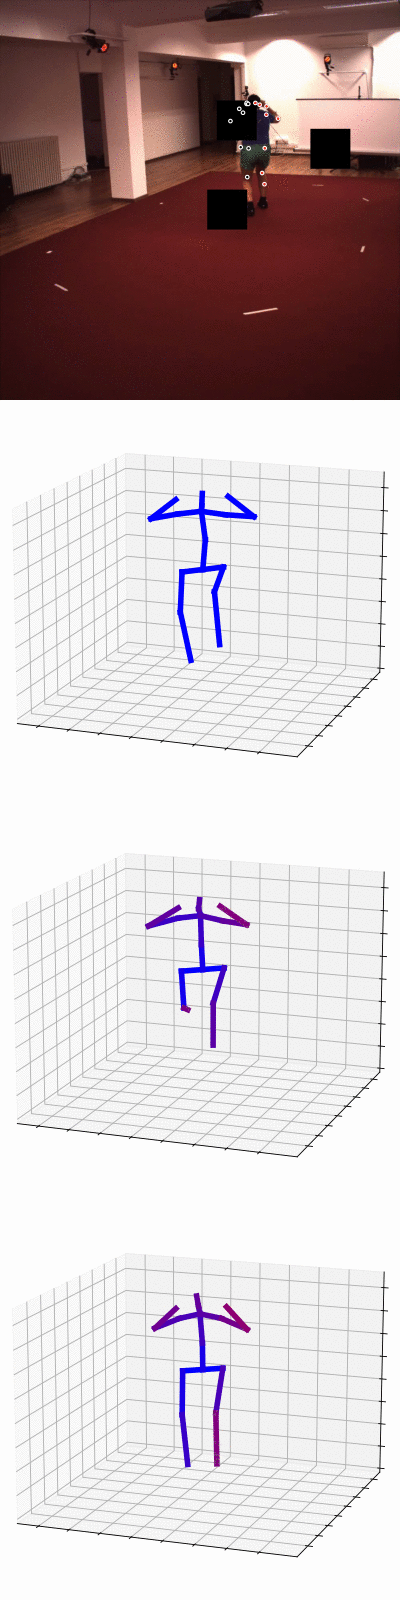}};
        \draw (\w * 9, \h * \r) node[inner sep=0] {\includegraphics[width=1.57cm]{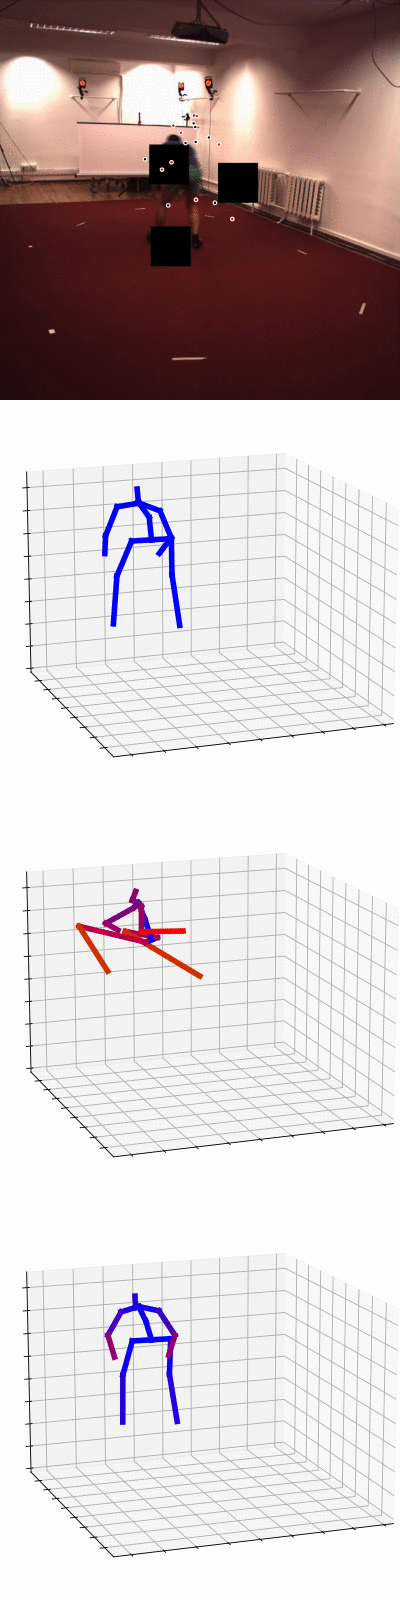}};
        
        \def \r{2}  
        \node at (-1.5, \h * \r - \u * 4 , 0) [below, rotate=90] {\footnotesize{VP3D + }};
        \node at (-1.25, \h * \r - \u * 4, 0) [below, rotate=90] {\footnotesize{TAGN}};
        \node at (-1.375, \h * \r - \u * 1.5, 0) [below, rotate=90] {\footnotesize{VP3D}};
        \node at (-1.375, \h * \r + \u * 1.2, 0) [below, rotate=90] {\footnotesize{GT}};
        \node at (-1.375, \h * \r + \u * 4,  0) [below, rotate=90] {\footnotesize{Frame}};
        \draw (\w * 0, \h * \r) node[inner sep=0] {\includegraphics[width=1.57cm]{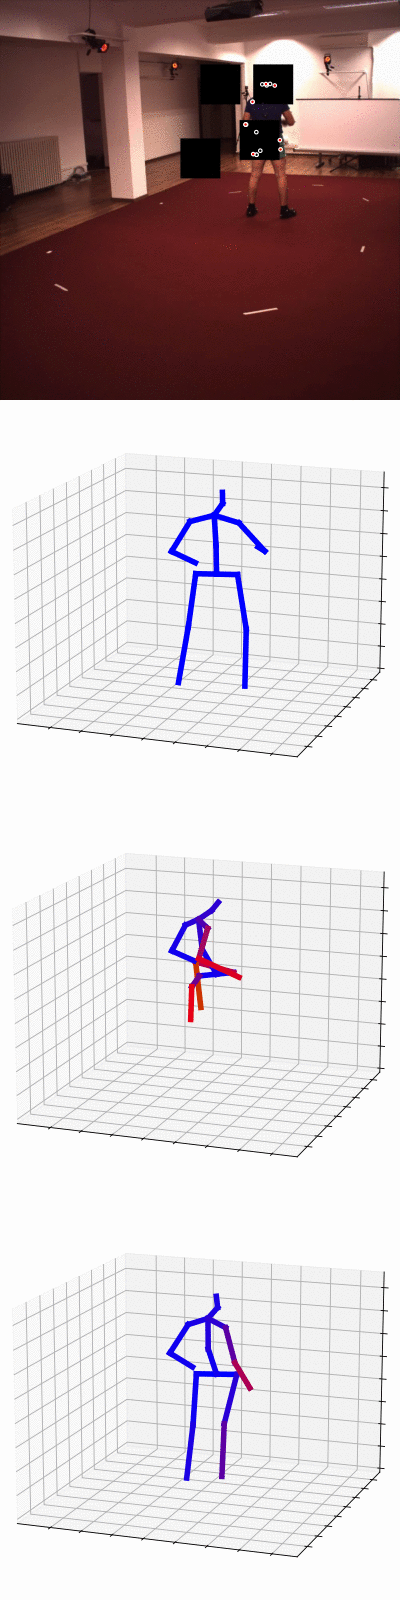}};
        \draw (\w * 1, \h * \r)node[inner sep=0]  {\includegraphics[width=1.57cm]{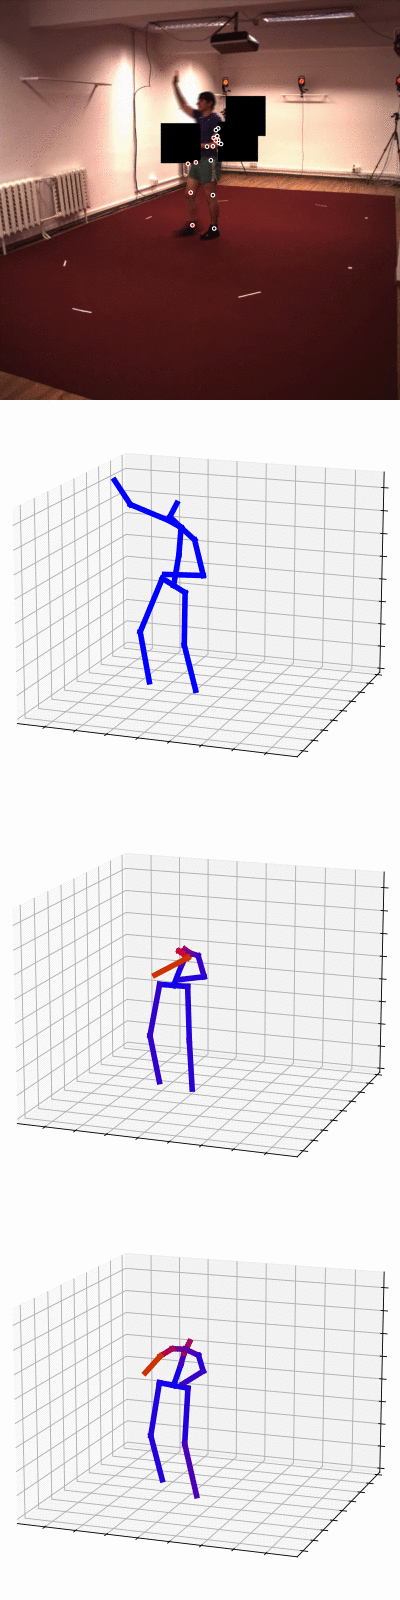}};
        \draw (\w * 2, \h * \r) node[inner sep=0] {\includegraphics[width=1.57cm]{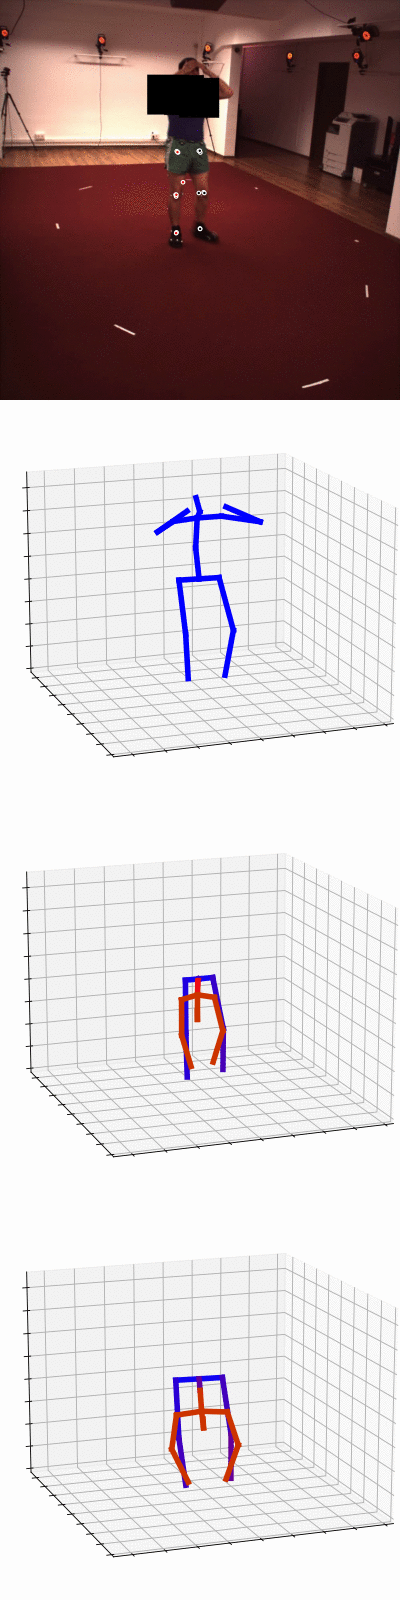}};
        \draw (\w * 3 ,\h * \r) node[inner sep=0] {\includegraphics[width=1.57cm]{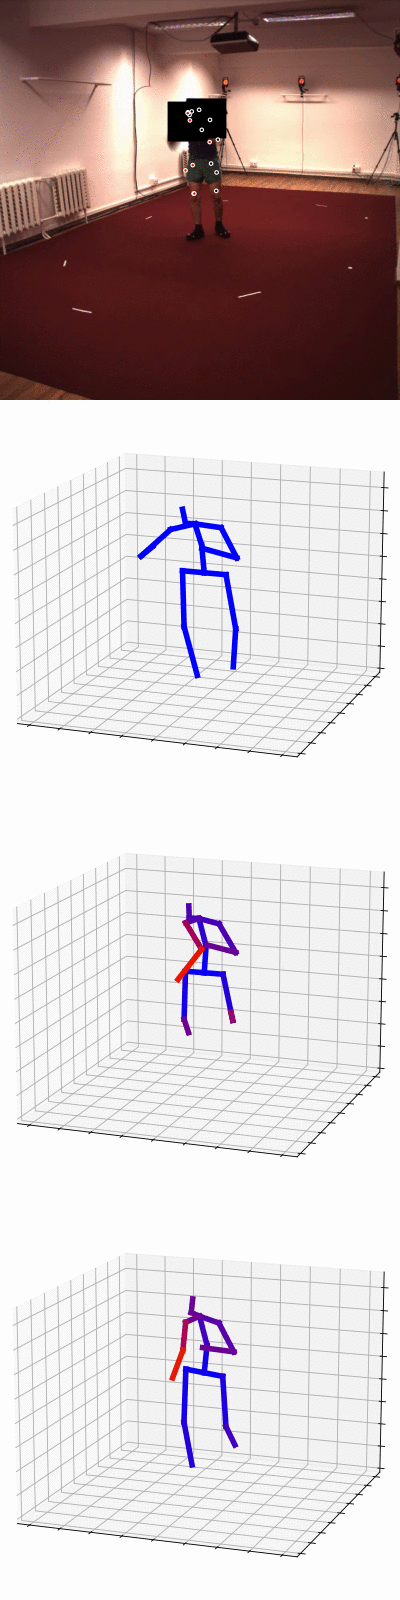}};
        \draw (\w * 4, \h * \r) node[inner sep=0] {\includegraphics[width=1.57cm]{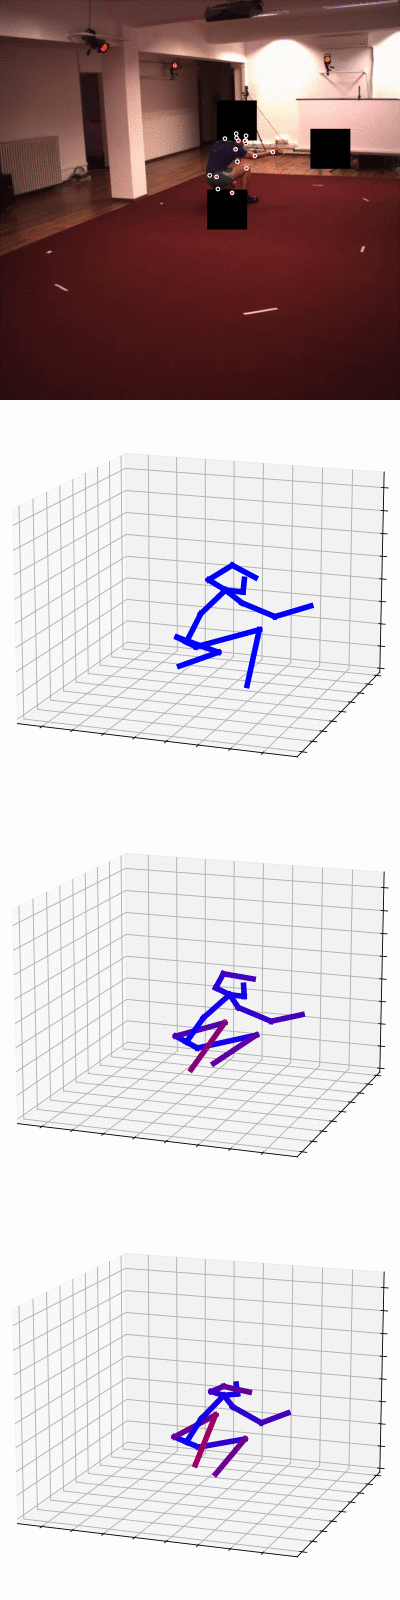}};
        \draw (\w * 5, \h * \r) node[inner sep=0] {\includegraphics[width=1.57cm]{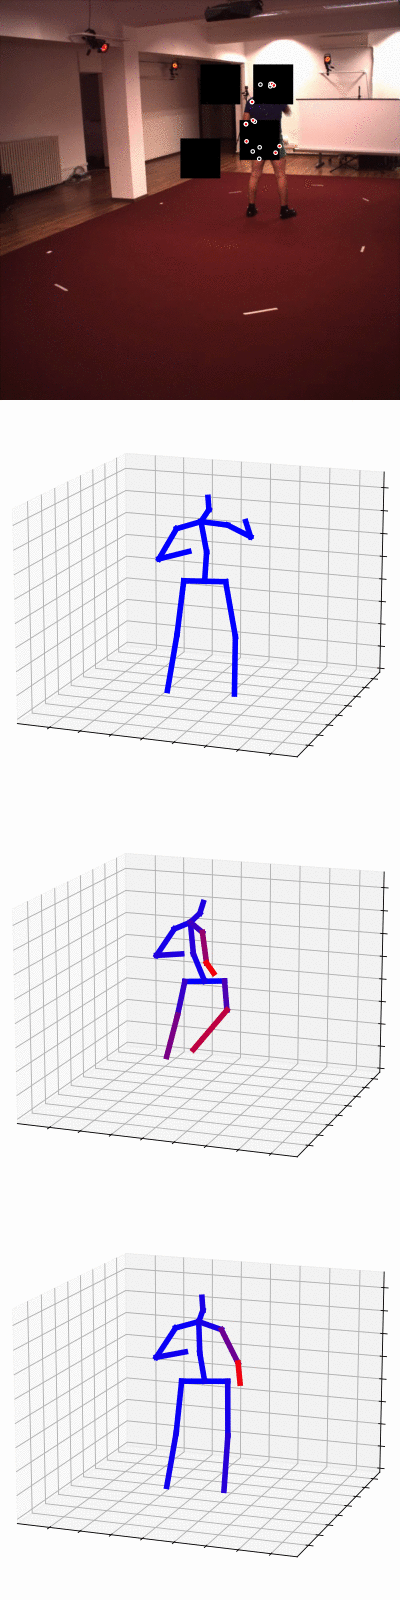}};
        \draw (\w * 6, \h * \r) node[inner sep=0] {\includegraphics[width=1.57cm]{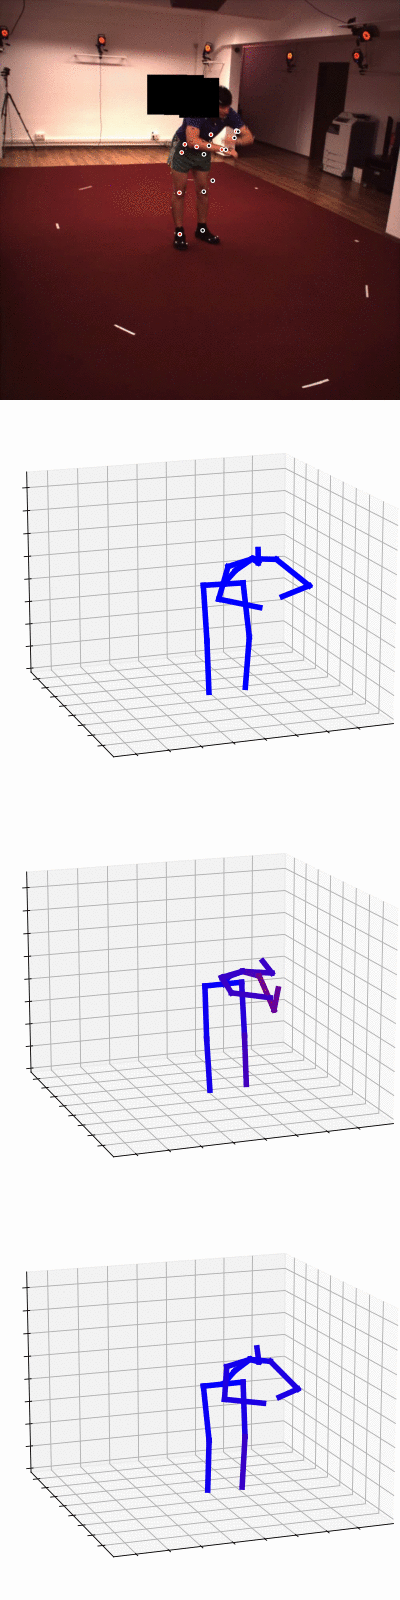}};
        \draw (\w * 7, \h * \r) node[inner sep=0] {\includegraphics[width=1.57cm]{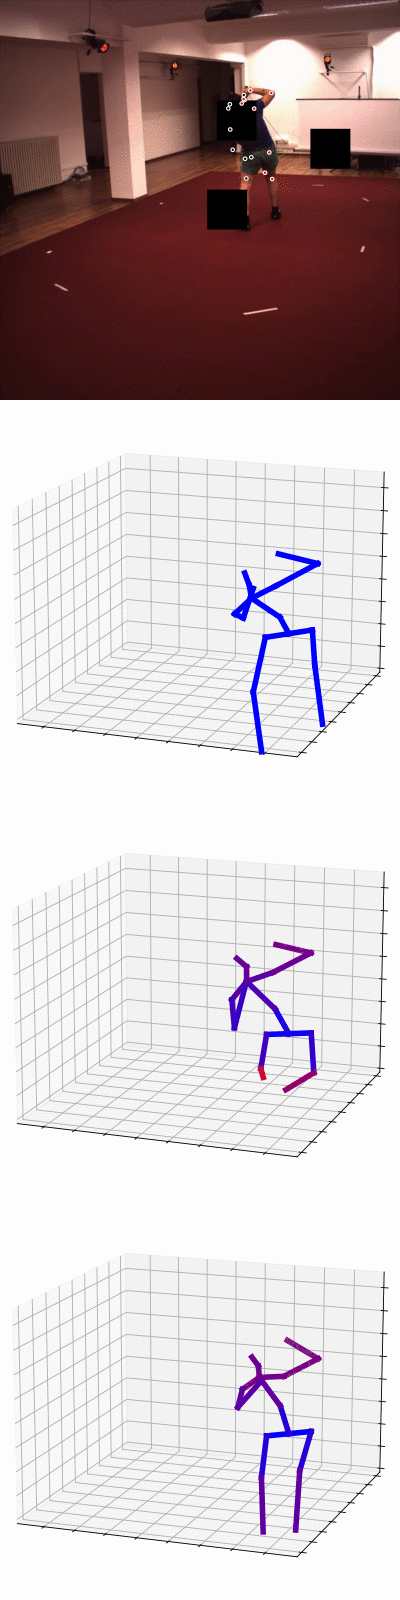}};
        \draw (\w * 8, \h * \r) node[inner sep=0] {\includegraphics[width=1.57cm]{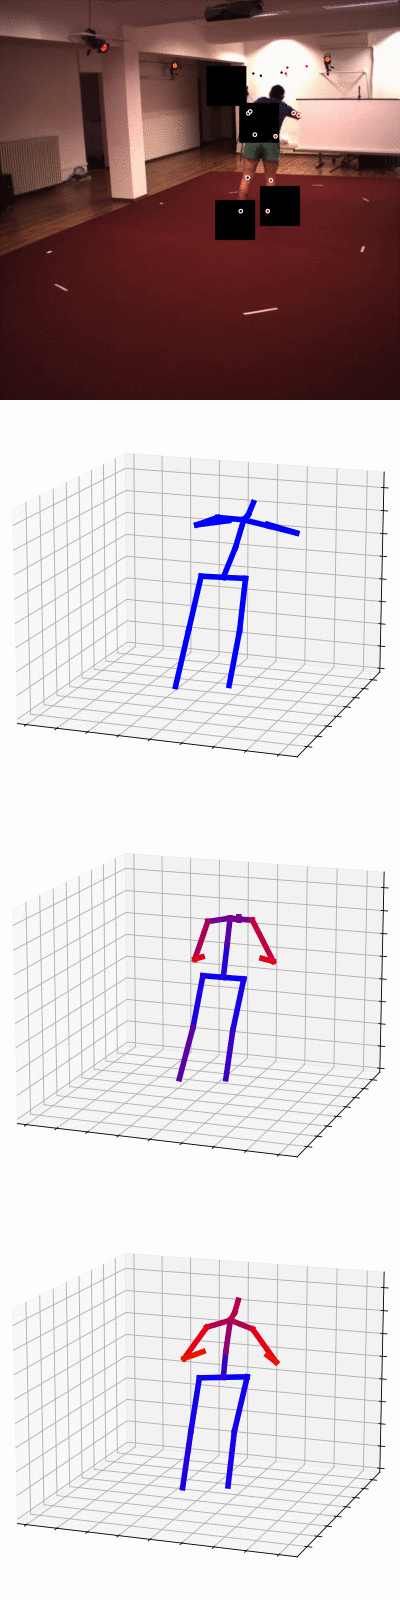}};
        \draw (\w * 9, \h * \r) node[inner sep=0] {\includegraphics[width=1.57cm]{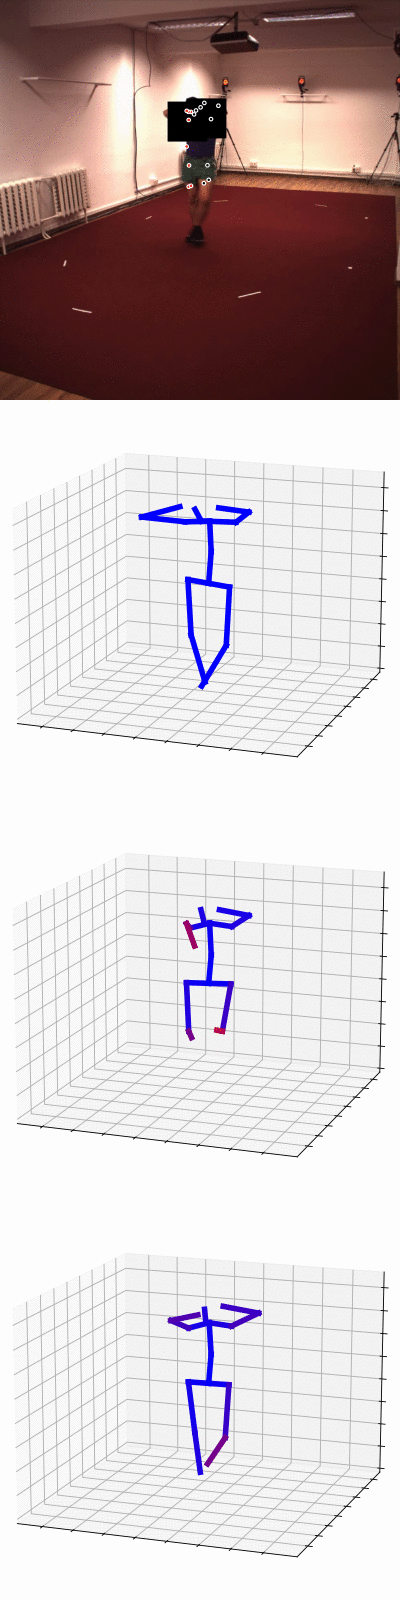}};

        \end{tikzpicture}
    \vspace*{-0.5\baselineskip}
    \caption{Qualitative comparison of VP3D+TAGN ($\sigma=0.3, p=k=50\%$) versus VP3D, on H36M-C dataset (with guided-patch erasing corruption). The bone color leading to a joint turns \textcolor{red}{red} when its MPJPE increases.}
    \vspace*{-\baselineskip}
    \label{fig:supp-tagn-qualitative}
\end{figure*}
